# Supplementary material for: The QUEST Database of Highly-Accurate Excitation Energies
Source: arXiv:2506.11590 ancillary file (2025-07-28)
Supplement: Supplementary file 1 [file QUEST-SI-Geom.pdf]

# SI for The QUEST Database of Highly-Accurate Excitation Energies: Geometries

Pierre-François Loos,*,† Martial Boggio-Pasqua,† Aymeric Blondel,‡ Filippo Lipparini,¶ and Denis Jacquemin*,‡,§

†*Laboratoire de Chimie et Physique Quantiques, Université de Toulouse, CNRS, F-31062 Toulouse, France*

‡*Nantes Université, CNRS, CEISAM UMR 6230, F-44000 Nantes, France*

¶*Dipartimento di Chimica e Chimica Industriale, University of Pisa, Via Moruzzi 3, 56124 Pisa, Italy*

§*Institut Universitaire de France (IUF), F-75005 Paris, France*

E-mail: loos@irsamc.ups-tlse.fr; Denis.Jacquemin@univ-nantes.fr

Below are given the Cartesian coordinates of the compounds investigated in this study. All structures are given in au (bohrs).

# S1 MAIN subset

## S1.1 Acetaldehyde

CASRN: 75-07-0

Level of theory: CC3(Full)/*aug*-cc-pVTZ

```
C   -0.00234503    0.00000000    0.87125063
C   -1.75847785    0.00000000   -1.34973671
O    2.27947397    0.00000000    0.71968028
H   -0.92904537    0.00000000    2.73929404
H   -2.97955463    1.66046488   -1.25209463
H   -2.97955463   -1.66046488   -1.25209463
H   -0.70043433    0.00000000   -3.11066412
```

## S1.2 Acetone

CASRN: 67-64-1

Level of theory: CC3(Full)/*aug*-cc-pVTZ

```
C    0.00000000    0.00000000    0.18807702
C    0.00000000    2.42007545   -1.31764698
C    0.00000000   -2.42007545   -1.31764698
O    0.00000000    0.00000000    2.48269094
H    0.00000000    4.03690733   -0.05185132
H    0.00000000   -4.03690733   -0.05185132
H    1.66061256    2.48420530   -2.53995285
H   -1.66061256    2.48420530   -2.53995285
H    1.66061256   -2.48420530   -2.53995285
H   -1.66061256   -2.48420530   -2.53995285
```

## S1.3 Acetylene

CASRN: 74-86-2

Level of theory: CC3(Full)/*aug*-cc-pVTZ

Ground state

```
C    0.00000000    0.00000000    1.14048351
C    0.00000000    0.00000000   -1.14048351
```

| | | | |
|---|---|---|---|
| H | 0.00000000 | 0.00000000 | 3.14009043 |
| H | 0.00000000 | 0.00000000 | -3.14009043 |

*Trans* excited state ($^1A_u$ state in the $C_{2h}$ point group)

| | | | |
|---|---|---|---|
| C | 1.29567779 | 0.00000000 | -0.01846047 |
| C | -1.29567779 | 0.00000000 | 0.01846047 |
| H | 2.41938674 | 0.00000000 | 1.70881682 |
| H | -2.41938674 | 0.00000000 | -1.70881682 |

*Cis* excited state ($^1A_2$ state in the $C_{2v}$ point group)

| | | | |
|---|---|---|---|
| C | 0.00000000 | 1.26834508 | -0.11726146 |
| C | 0.00000000 | -1.26834508 | -0.11726146 |
| H | 0.00000000 | 2.67282325 | 1.39629264 |
| H | 0.00000000 | -2.67282325 | 1.39629264 |

## S1.4 Acrolein

CASRN: 107-02-8

Level of theory: CC3(Full)/*aug*-cc-pVTZ

| | | | |
|---|---|---|---|
| C | -1.11645072 | -0.68348783 | 0.00000000 |
| C | 1.20647847 | 0.83714564 | 0.00000000 |
| C | 3.46831059 | -0.28872636 | 0.00000000 |
| O | -3.23666415 | 0.19187203 | 0.00000000 |
| H | -0.80613858 | -2.74747338 | 0.00000000 |
| H | 0.98699813 | 2.86613511 | 0.00000000 |
| H | 5.20930864 | 0.77443560 | 0.00000000 |
| H | 3.60951559 | -2.33000749 | 0.00000000 |

## S1.5 Aminobenzonitrile

CASRN: 873-74-5 (4-Aminobenzonitrile)

Level of theory: CC3(FC)/cc-pVTZ

| | | | |
|---|---|---|---|
| C | 0.00000000 | 0.00000000 | -3.36820633 |
| C | 2.27829762 | 0.00000000 | -2.01450309 |
| C | -2.27829762 | 0.00000000 | -2.01450309 |
| C | 0.00000000 | 0.00000000 | 1.93909521 |
| C | 2.27351166 | 0.00000000 | 0.59753796 |

| | | | |
|---|---|---|---|
| C | -2.27351166 | 0.00000000 | 0.59753796 |
| C | 0.00000000 | 0.00000000 | 4.63257112 |
| N | 0.00000000 | 0.00000000 | -5.94870080 |
| N | 0.00000000 | 0.00000000 | 6.83060124 |
| H | 4.04775542 | 0.00000000 | -3.02611570 |
| H | -4.04775542 | 0.00000000 | -3.02611570 |
| H | 4.03704439 | 0.00000000 | 1.61551747 |
| H | -4.03704439 | 0.00000000 | 1.61551747 |
| H | -1.62177115 | 0.00000000 | -6.91608217 |
| H | 1.62177115 | 0.00000000 | -6.91608217 |

## S1.6 Ammonia

CASRN: 7664-41-7

Level of theory: CC3(Full)/*aug*-cc-pVTZ

| | | | |
|---|---|---|---|
| N | 0.12804615 | 0.00000000 | 0.00000000 |
| H | -0.59303935 | 0.88580079 | -1.53425197 |
| H | -0.59303935 | -1.77160157 | 0.00000000 |
| H | -0.59303935 | 0.88580079 | 1.53425197 |

## S1.7 Aniline

CASRN: 62-53-3

Level of theory: CC3(FC)/cc-pVTZ – $C_{2v}$ enforced

| | | | |
|---|---|---|---|
| C | 0.00000000 | 0.00000000 | -1.78643569 |
| C | 2.27316118 | 0.00000000 | -0.43457234 |
| C | -2.27316118 | 0.00000000 | -0.43457234 |
| C | 0.00000000 | 0.00000000 | 3.53007775 |
| C | 2.26327651 | 0.00000000 | 2.18912925 |
| C | -2.26327651 | 0.00000000 | 2.18912925 |
| N | 0.00000000 | 0.00000000 | -4.38230793 |
| H | 4.03982526 | 0.00000000 | 3.18807501 |
| H | -4.03982526 | 0.00000000 | 3.18807501 |
| H | 0.00000000 | 0.00000000 | 5.56493193 |
| H | 4.04200589 | 0.00000000 | -1.45016965 |
| H | -4.04200589 | 0.00000000 | -1.45016965 |
| H | -1.62137595 | 0.00000000 | -5.34754284 |
| H | 1.62137595 | 0.00000000 | -5.34754284 |

## S1.8 Azanaphthalene

CASRN: 255-53-8 (Pyrazino[2,3-*b*]pyrazine or 1,4,5,8-Tetraazanaphthalene)

Level of theory: CC3(Full)/cc-pVTZ

| | | | |
|---|---|---|---|
| C | 0.00000000 | 1.33735978 | 0.00000000 |
| C | 0.00000000 | -1.33735978 | 0.00000000 |
| C | 4.26447087 | 1.34122299 | 0.00000000 |
| C | -4.26447087 | 1.34122299 | 0.00000000 |
| C | 4.26447087 | -1.34122299 | 0.00000000 |
| C | -4.26447087 | -1.34122299 | 0.00000000 |
| N | 2.18301381 | 2.68816340 | 0.00000000 |
| N | -2.18301381 | 2.68816340 | 0.00000000 |
| N | 2.18301381 | -2.68816340 | 0.00000000 |
| N | -2.18301381 | -2.68816340 | 0.00000000 |
| H | 6.03657953 | 2.35467535 | 0.00000000 |
| H | -6.03657953 | 2.35467535 | 0.00000000 |
| H | 6.03657953 | -2.35467535 | 0.00000000 |
| H | -6.03657953 | -2.35467535 | 0.00000000 |

## S1.9 Azulene

CASRN: 275-51-4

Level of theory: CC3(FC)/cc-pVTZ

| | | | |
|---|---|---|---|
| C | 0.00000000 | 0.00000000 | -5.08442654 |
| C | 2.16799436 | 0.00000000 | -3.55850254 |
| C | -2.16799436 | 0.00000000 | -3.55850254 |
| C | 1.40560615 | 0.00000000 | -1.02382432 |
| C | -1.40560615 | 0.00000000 | -1.02382432 |
| C | 0.00000000 | 0.00000000 | 4.72891515 |
| C | 2.38587647 | 0.00000000 | 3.61219185 |
| C | -2.38587647 | 0.00000000 | 3.61219185 |
| C | 3.00158451 | 0.00000000 | 1.05184313 |
| C | -3.00158451 | 0.00000000 | 1.05184313 |
| H | 0.00000000 | 0.00000000 | -7.11850559 |
| H | 4.09656030 | 0.00000000 | -4.20278074 |
| H | -4.09656030 | 0.00000000 | -4.20278074 |
| H | 0.00000000 | 0.00000000 | 6.77201689 |
| H | 3.96514987 | 0.00000000 | 4.90481753 |
| H | -3.96514987 | 0.00000000 | 4.90481753 |
| H | 5.00047162 | 0.00000000 | 0.61482964 |
| H | -5.00047162 | 0.00000000 | 0.61482964 |

## S1.10 Benzene

CASRN: 71-43-2

Level of theory: CC3(Full)/*aug*-cc-pVTZ

| | | | |
|---|---|---|---|
| C | 0.00000000 | 2.63144965 | 0.00000000 |
| C | -2.27890225 | 1.31572483 | 0.00000000 |
| C | -2.27890225 | -1.31572483 | 0.00000000 |
| C | 0.00000000 | -2.63144965 | 0.00000000 |
| C | 2.27890225 | -1.31572483 | 0.00000000 |
| C | 2.27890225 | 1.31572483 | 0.00000000 |
| H | -4.04725813 | 2.33668557 | 0.00000000 |
| H | -4.04725813 | -2.33668557 | 0.00000000 |
| H | 0.00000000 | -4.67337115 | 0.00000000 |
| H | 4.04725813 | -2.33668557 | 0.00000000 |
| H | 4.04725813 | 2.33668557 | 0.00000000 |
| H | 0.00000000 | 4.67337115 | 0.00000000 |

## S1.11 Benzonitrile

CASRN: 100-47-0

Level of theory: CC3(FC)/cc-pVTZ

| | | | |
|---|---|---|---|
| C | 0.00000000 | 0.00000000 | -3.73018216 |
| C | 0.00000000 | 0.00000000 | -1.02720486 |
| C | 2.28760421 | 0.00000000 | 0.28592358 |
| C | -2.28760421 | 0.00000000 | 0.28592358 |
| C | 0.00000000 | 0.00000000 | 4.22270922 |
| C | 2.28059554 | 0.00000000 | 2.90986462 |
| C | -2.28059554 | 0.00000000 | 2.90986462 |
| N | 0.00000000 | 0.00000000 | -5.92640038 |
| H | 4.03930466 | 0.00000000 | -0.75078588 |
| H | -4.03930466 | 0.00000000 | -0.75078588 |
| H | 4.04556576 | 0.00000000 | 3.92452034 |
| H | -4.04556576 | 0.00000000 | 3.92452034 |
| H | 0.00000000 | 0.00000000 | 6.25892556 |

## S1.12 Benzoquinone

CASRN: 106-51-4 (1,4-Benzoquinone)

Level of theory: CC3(Full)/*aug*-cc-pVTZ

| | | | |
|---|---|---|---|
| C | 2.71467427 | 0.00000000 | 0.00000000 |
| C | -2.71467427 | 0.00000000 | 0.00000000 |
| C | 1.26645689 | 2.38719964 | 0.00000000 |
| C | 1.26645689 | -2.38719964 | 0.00000000 |
| C | -1.26645689 | 2.38719964 | 0.00000000 |
| C | -1.26645689 | -2.38719964 | 0.00000000 |
| O | 5.02607647 | 0.00000000 | 0.00000000 |
| O | -5.02607647 | 0.00000000 | 0.00000000 |
| H | 2.37218673 | 4.10318853 | 0.00000000 |
| H | 2.37218673 | -4.10318853 | 0.00000000 |
| H | -2.37218673 | 4.10318853 | 0.00000000 |
| H | -2.37218673 | -4.10318853 | 0.00000000 |

## S1.13 Benzothiadiazole

CASRN: 273-13-2 (2,1,3-Benzothiadiazole)

Level of theory: CC3(FC)/cc-pVTZ

| | | | |
|---|---|---|---|
| S | 0.00000000 | 0.00000000 | 4.12782363 |
| N | 0.00000000 | 2.37994968 | 2.16794907 |
| N | 0.00000000 | -2.37994968 | 2.16794907 |
| C | 0.00000000 | 1.35464582 | -0.15090868 |
| C | 0.00000000 | -1.35464582 | -0.15090868 |
| C | 0.00000000 | 2.70608821 | -2.46599859 |
| C | 0.00000000 | -2.70608821 | -2.46599859 |
| C | 0.00000000 | 1.34964552 | -4.66429754 |
| C | 0.00000000 | -1.34964552 | -4.66429754 |
| H | 0.00000000 | 4.74051264 | -2.44976392 |
| H | 0.00000000 | -4.74051264 | -2.44976392 |
| H | 0.00000000 | 2.32640888 | -6.45161040 |
| H | 0.00000000 | -2.32640888 | -6.45161040 |

## S1.14 Benzoxadiazole

CASRN: 273-09-6 (2,1,3-Benzoxadiazole)

Level of theory: CC3(FC)/cc-pVTZ

| | | | |
|---|---|---|---|
| O | 0.00000000 | 0.00000000 | 4.23105351 |
| N | 0.00000000 | 2.15721782 | 2.80042430 |
| N | 0.00000000 | -2.15721782 | 2.80042430 |
| C | 0.00000000 | 1.34474119 | 0.44505130 |

| | | | |
|---|---|---|---|
| C | 0.00000000 | -1.34474119 | 0.44505130 |
| C | 0.00000000 | 2.73330026 | -1.85469062 |
| C | 0.00000000 | -2.73330026 | -1.85469062 |
| C | 0.00000000 | 1.35965956 | -4.03354365 |
| C | 0.00000000 | -1.35965956 | -4.03354365 |
| H | 0.00000000 | 4.76633138 | -1.84544064 |
| H | 0.00000000 | -4.76633138 | -1.84544064 |
| H | 0.00000000 | 2.32124878 | -5.82853313 |
| H | 0.00000000 | -2.32124878 | -5.82853313 |

## S1.15 Beryllium

CASRN: 7440-41-7

Level of theory: N/A

| | | | |
|---|---|---|---|
| Be | 0.00000000 | 0.00000000 | 0.00000000 |

## S1.16 BF

CASRN: 13768-60-0 (Boron fluoride)

Level of theory: CC3(Full)/*aug*-cc-pVTZ

| | | | |
|---|---|---|---|
| B | 0.00000000 | 0.00000000 | 0.00000000 |
| F | 0.00000000 | 0.00000000 | 2.39729626 |

## S1.17 BH

CASRN: 13766-26-2 (Boron hydride or borane)

Level of theory: CC3(Full)/*aug*-cc-pVTZ

Ground state

| | | | |
|---|---|---|---|
| B | 0.00000000 | 0.00000000 | 0.00000000 |
| H | 0.00000000 | 0.00000000 | 2.31089693 |

Excited state

| | | | |
|---|---|---|---|
| B | 0.00000000 | 0.00000000 | 0.00000000 |
| H | 0.00000000 | 0.00000000 | 2.27596436 |

## S1.18 Borole

CASRN: 287-87-6

Level of theory: CC3(Full)/*aug*-cc-pVTZ

| | | | |
|---|---|---|---|
| B | 0.00000000 | 0.00000000 | 2.44991435 |
| C | 0.00000000 | 2.35991046 | 0.62561328 |
| C | 0.00000000 | -2.35991046 | 0.62561328 |
| C | 0.00000000 | 1.42526648 | -1.74135978 |
| C | 0.00000000 | -1.42526648 | -1.74135978 |
| H | 0.00000000 | 0.00000000 | 4.69246473 |
| H | 0.00000000 | 4.35732912 | 1.03002724 |
| H | 0.00000000 | -4.35732912 | 1.03002724 |
| H | 0.00000000 | 2.51021632 | -3.47247633 |
| H | 0.00000000 | -2.51021632 | -3.47247633 |

## S1.19 Butadiene

CASRN: 106-99-0

Level of theory: CC3(Full)/*aug*-cc-pVTZ

| | | | |
|---|---|---|---|
| C | 1.14656244 | 0.00000000 | 0.75468820 |
| C | -1.14656244 | 0.00000000 | -0.75468820 |
| C | 3.48132647 | 0.00000000 | -0.22482805 |
| C | -3.48132647 | 0.00000000 | 0.22482805 |
| H | 0.90770978 | 0.00000000 | 2.78883925 |
| H | -0.90770978 | 0.00000000 | -2.78883925 |
| H | 3.77525814 | 0.00000000 | -2.24895470 |
| H | -3.77525814 | 0.00000000 | 2.24895470 |
| H | 5.13664967 | 0.00000000 | 0.96861890 |
| H | -5.13664967 | 0.00000000 | -0.96861890 |

## S1.20 Carbon dimer

CASRN: 12070-15-4 (1,2-Ethynediyl)

Level of theory: CC3(Full)/*aug*-cc-pVTZ

| | | | |
|---|---|---|---|
| C | 0.00000000 | 0.00000000 | 1.17922927 |
| C | 0.00000000 | 0.00000000 | -1.17922927 |

## S1.21 Carbon dioxide

CASRN: 124-38-9

Level of theory: CC3(FC)/*aug*-cc-pVTZ

| | | | |
|---|---|---|---|
| C | 0.00000000 | 0.00000000 | 0.00000000 |
| O | 0.00000000 | 0.00000000 | -2.20193016 |
| O | 0.00000000 | 0.00000000 | 2.20193016 |

## S1.22 Carbonic acid

CASRN: 463-79-6

Level of theory: CC3(FC)/*aug*-cc-pVTZ

| | | | |
|---|---|---|---|
| O | 0.00000000 | 0.00000000 | 2.46279243 |
| C | 0.00000000 | 0.00000000 | 0.18750328 |
| O | 0.00000000 | 2.04786599 | -1.29140793 |
| O | 0.00000000 | -2.04786599 | -1.29140793 |
| H | 0.00000000 | 3.47810449 | -0.16385522 |
| H | 0.00000000 | -3.47810449 | -0.16385522 |

## S1.23 Carbon monoxide

CASRN: 630-08-0

Level of theory: CC3(Full)/*aug*-cc-pVTZ

| | | | |
|---|---|---|---|
| C | 0.00000000 | 0.00000000 | -1.24942055 |
| O | 0.00000000 | 0.00000000 | 0.89266692 |

## S1.24 Carbon trimer

CASRN: 12075-35-3 (1,2-Propadiene-1,3-diylidene)

Level of theory: CC3(Full)/*aug*-cc-pVTZ

| | | | |
|---|---|---|---|
| C | 0.00000000 | 0.00000000 | 0.00000000 |
| C | 0.00000000 | 0.00000000 | 2.45345613 |
| C | 0.00000000 | 0.00000000 | -2.45345613 |

## S1.25 Carbonyl fluoride

CASRN: 353-50-4

Level of theory: CC3(Full)/*aug*-cc-pVTZ

| | | | |
|---|---|---|---|
| C | 0.00000000 | 0.00000000 | -0.30652633 |
| O | 0.00000000 | 0.00000000 | -2.52469534 |
| F | 0.00000000 | 2.00254958 | 1.16003038 |
| F | 0.00000000 | -2.00254958 | 1.16003038 |

## S1.26 $CCl_2$

CASRN: 1605-72-7 (Dichlorocarbene)

Level of theory: CC3(Full)/*aug*-cc-pVTZ

| | | | |
|---|---|---|---|
| C | 0.00000000 | 0.00000000 | -1.60920674 |
| Cl | 0.00000000 | 2.65360612 | 0.27602958 |
| Cl | 0.00000000 | -2.65360612 | 0.27602958 |

## S1.27 CClF

CASRN: 1691-88-9 (Chlorofluorocarbene)

Level of theory: CC3(Full)/*aug*-cc-pVTZ

| | | | |
|---|---|---|---|
| C | 0.29776085 | 0.00000000 | 1.47969075 |
| F | 2.16980264 | 0.00000000 | -0.10569879 |
| Cl | -2.46756349 | 0.00000000 | -0.32822320 |

## S1.28 $CF_2$

CASRN: 2154-59-8 (Difluorocarbene)

Level of theory: CC3(Full)/*aug*-cc-pVTZ

| | | | |
|---|---|---|---|
| C | 0.00000000 | 0.00000000 | -1.14170749 |
| F | 0.00000000 | 1.94810617 | 0.36114458 |
| F | 0.00000000 | -1.94810617 | 0.36114458 |

## S1.29 Chlorobenzene

CASRN: 108-90-7

Level of theory: CC3(FC)/cc-pVTZ

| | | | |
|---|---|---|---|
| Cl | 0.00000000 | 0.00000000 | -4.09694569 |
| C | 0.00000000 | 0.00000000 | -0.80648356 |
| C | 2.28704058 | 0.00000000 | 0.47978453 |
| C | -2.28704058 | 0.00000000 | 0.47978453 |
| C | 0.00000000 | 0.00000000 | 4.42840669 |
| C | 2.27492426 | 0.00000000 | 3.10862132 |
| C | -2.27492426 | 0.00000000 | 3.10862132 |
| H | 4.03299260 | 0.00000000 | -0.56250521 |
| H | -4.03299260 | 0.00000000 | -0.56250521 |
| H | 4.04398612 | 0.00000000 | 4.11768561 |
| H | -4.04398612 | 0.00000000 | 4.11768561 |
| H | 0.00000000 | 0.00000000 | 6.46409111 |

## S1.30 Criegee's Intermediate

CASRN: 56077-92-0 (Formaldehyde oxide)

Level of theory: CC3(Full)/*aug*-cc-pVTZ

| | | | |
|---|---|---|---|
| C | -2.14193693 | 0.46449461 | 0.00000000 |
| O | -0.12214743 | -0.85046436 | 0.00000000 |
| O | 2.09779397 | 0.38347786 | 0.00000000 |
| H | -3.86593284 | -0.61908241 | 0.00000000 |
| H | -1.98533536 | 2.49983926 | 0.00000000 |

## S1.31 Cyanoacetylene

CASRN: 1070-71-9

Level of theory: CC3(Full)/*aug*-cc-pVTZ

Ground state

| | | | |
|---|---|---|---|
| C | 0.00000000 | 0.00000000 | -3.59120182 |
| C | 0.00000000 | 0.00000000 | -1.30693904 |
| C | 0.00000000 | 0.00000000 | 1.28880240 |
| N | 0.00000000 | 0.00000000 | 3.48692211 |
| H | 0.00000000 | 0.00000000 | -5.59619886 |

Lowest excited state

| | | | |
|---|---|---|---|
| C | 1.99411175 | 0.00000000 | 2.81781077 |
| C | -0.07304269 | 0.00000000 | 1.33125774 |
| C | -0.63630126 | 0.00000000 | -1.14556678 |
| N | -1.39755756 | 0.00000000 | -3.26154643 |
| H | 1.90749857 | 0.00000000 | 4.87279180 |

## S1.32 Cyanoformaldehyde

CASRN: 4471-47-0

Level of theory: CC3(Full)/*aug*-cc-pVTZ

| | | | |
|---|---|---|---|
| C | -0.91561483 | 0.00000000 | -1.22522833 |
| C | -0.01092219 | 0.00000000 | 1.39523175 |
| N | 0.64170259 | 0.00000000 | 3.48820325 |
| O | 0.50833684 | 0.00000000 | -3.00337867 |
| H | -2.97202213 | 0.00000000 | -1.42565674 |

## S1.33 Cyanogen

CASRN: 460-19-5 (Ethanedinitrile)

Level of theory: CC3(Full)/*aug*-cc-pVTZ

Ground state

| | | | |
|---|---|---|---|
| C | 0.00000000 | 0.00000000 | 1.30401924 |
| C | 0.00000000 | 0.00000000 | -1.30401924 |
| N | 0.00000000 | 0.00000000 | 3.49784121 |
| N | 0.00000000 | 0.00000000 | -3.49784121 |

Excited state

| | | | |
|---|---|---|---|
| C | 0.00000000 | 0.00000000 | 1.22784115 |
| C | 0.00000000 | 0.00000000 | -1.22784115 |
| N | 0.00000000 | 0.00000000 | 3.56462559 |
| N | 0.00000000 | 0.00000000 | -3.56462559 |

## S1.34 Cyclobutadiene

CASRN: 1120-53-2

Level of theory: CC3(Full)/*aug*-cc-pVTZ

| | | | |
|---|---|---|---|
| C | -1.47868321 | -1.27004715 | 0.00000000 |
| C | 1.47868321 | -1.27004715 | 0.00000000 |
| C | -1.47868321 | 1.27004715 | 0.00000000 |
| C | 1.47868321 | 1.27004715 | 0.00000000 |
| H | -2.91448237 | -2.70994518 | 0.00000000 |
| H | 2.91448237 | -2.70994518 | 0.00000000 |
| H | -2.91448237 | 2.70994518 | 0.00000000 |
| H | 2.91448237 | 2.70994518 | 0.00000000 |

## S1.35 Cyclopentadiene

CASRN: 542-92-7

Level of theory: CC3(Full)/*aug*-cc-pVTZ

| | | | |
|---|---|---|---|
| C | 0.00000000 | 0.00000000 | -2.33113051 |
| C | 0.00000000 | 2.22209092 | -0.56871188 |
| C | 0.00000000 | -2.22209092 | -0.56871188 |
| C | 0.00000000 | 1.38514451 | 1.83772922 |
| C | 0.00000000 | -1.38514451 | 1.83772922 |
| H | 1.66130504 | 0.00000000 | -3.56414299 |
| H | -1.66130504 | 0.00000000 | -3.56414299 |
| H | 0.00000000 | 4.16550405 | -1.18116624 |
| H | 0.00000000 | -4.16550405 | -1.18116624 |
| H | 0.00000000 | 2.54514584 | 3.51352303 |
| H | 0.00000000 | -2.54514584 | 3.51352303 |

## S1.36 Cyclopentadienethione

CASRN: 77825-99-1 (2,4-Cyclopentadiene-1-thione)

Level of theory: CC3(Full)/*aug*-cc-pVTZ

| | | | |
|---|---|---|---|
| C | 0.00000000 | 0.00000000 | 0.54718884 |
| C | 0.00000000 | 2.23394142 | -1.11648863 |
| C | 0.00000000 | -2.23394142 | -1.11648863 |
| C | 0.00000000 | 1.40618242 | -3.52381930 |
| C | 0.00000000 | -1.40618242 | -3.52381930 |
| S | 0.00000000 | 0.00000000 | 3.63323789 |
| H | 0.00000000 | 4.14572930 | -0.42732005 |
| H | 0.00000000 | -4.14572930 | -0.42732005 |
| H | 0.00000000 | 2.55090221 | -5.20908210 |
| H | 0.00000000 | -2.55090221 | -5.20908210 |

## S1.37 Cyclopentadienone

CASRN: 13177-38-3 (2,4-Cyclopentadien-1-one)

Level of theory: CC3(Full)/*aug*-cc-pVTZ

| | | | |
|---|---|---|---|
| C | 0.00000000 | 0.00000000 | 1.45232781 |
| C | 0.00000000 | 2.26718523 | -0.25413145 |
| C | 0.00000000 | -2.26718523 | -0.25413145 |
| C | 0.00000000 | 1.41557636 | -2.63852689 |
| C | 0.00000000 | -1.41557636 | -2.63852689 |
| O | 0.00000000 | 0.00000000 | 3.74438847 |
| H | 0.00000000 | 4.18416912 | 0.42151096 |
| H | 0.00000000 | -4.18416912 | 0.42151096 |
| H | 0.00000000 | 2.53760914 | -4.33851399 |
| H | 0.00000000 | -2.53760914 | -4.33851399 |

## S1.38 Cyclopropene

CASRN: 2781-85-3

Level of theory: CC3(Full)/*aug*-cc-pVTZ

| | | | |
|---|---|---|---|
| C | 0.00000000 | 0.00000000 | -1.66820880 |
| C | 0.00000000 | 1.22523906 | 0.90681419 |
| C | 0.00000000 | -1.22523906 | 0.90681419 |
| H | 1.72255446 | 0.00000000 | -2.77881149 |
| H | -1.72255446 | 0.00000000 | -2.77881149 |
| H | 0.00000000 | 2.97844519 | 1.92076771 |
| H | 0.00000000 | -2.97844519 | 1.92076771 |

## S1.39 Cyclopropenethione

CASRN: 69903-36-2

Level of theory: CC3(Full)/*aug*-cc-pVTZ

| | | | |
|---|---|---|---|
| C | 0.00000000 | 1.26230744 | -2.86571925 |
| C | 0.00000000 | -1.26230744 | -2.86571925 |
| C | 0.00000000 | 0.00000000 | -0.49233236 |
| S | 0.00000000 | 0.00000000 | 2.57821680 |
| H | 0.00000000 | 2.97773331 | -3.95114059 |
| H | 0.00000000 | -2.97773331 | -3.95114059 |

## S1.40 Cyclopropenone

CASRN: 2961-80-0

Level of theory: CC3(Full)/*aug*-cc-pVTZ

| | | | |
|---|---|---|---|
| C | 0.00000000 | 1.27491826 | -1.86930519 |
| C | 0.00000000 | -1.27491826 | -1.86930519 |
| C | 0.00000000 | 0.00000000 | 0.51814554 |
| O | 0.00000000 | 0.00000000 | 2.79326776 |
| H | 0.00000000 | 2.92791371 | -3.05679837 |
| H | 0.00000000 | -2.92791371 | -3.05679837 |

## S1.41 Diacetylene

CASRN: 460-12-8

Level of theory: CC3(Full)/*aug*-cc-pVTZ

| | | | |
|---|---|---|---|
| C | 0.00000000 | 0.00000000 | 1.29447700 |
| C | 0.00000000 | 0.00000000 | -1.29447700 |
| C | 0.00000000 | 0.00000000 | 3.58448429 |
| C | 0.00000000 | 0.00000000 | -3.58448429 |
| H | 0.00000000 | 0.00000000 | 5.58943003 |
| H | 0.00000000 | 0.00000000 | -5.58943003 |

## S1.42 Diazete

CASRN: 287-42-3 (1,3-Diazete)

Level of theory: CC3(Full)/*aug*-cc-pVTZ

| | | | |
|---|---|---|---|
| C | 1.04088890 | 1.37023206 | 0.00000000 |
| C | -1.04088890 | -1.37023206 | 0.00000000 |
| N | 1.80420222 | -0.93584807 | 0.00000000 |
| N | -1.80420222 | 0.93584807 | 0.00000000 |
| H | 2.06402011 | 3.13844681 | 0.00000000 |
| H | -2.06402011 | -3.13844681 | 0.00000000 |

## S1.43 Diazirine

CASRN: 157-22-2 (3*H*-Diazirine)

Level of theory: CC3(Full)/*aug*-cc-pVTZ

| | | | |
|---|---|---|---|
| C | 0.00000000 | 0.00000000 | -0.26696099 |
| H | 0.00000000 | 1.75890895 | -1.28616478 |
| H | 0.00000000 | -1.75890895 | -1.28616479 |
| N | 1.16058100 | 0.00000000 | 2.27183007 |
| N | -1.16058100 | 0.00000000 | 2.27183007 |

## S1.44 Diazomethane

CASRN: 334-88-3

Level of theory: CC3(Full)/*aug*-cc-pVTZ

Ground state

| | | | |
|---|---|---|---|
| C | 0.00000000 | 0.00000000 | -2.30830005 |
| N | 0.00000000 | 0.00000000 | 0.14457890 |
| N | 0.00000000 | 0.00000000 | 2.29923216 |
| H | 0.00000000 | 1.79875201 | -3.24272317 |
| H | 0.00000000 | -1.79875201 | -3.24272317 |

Excited state

| | | | |
|---|---|---|---|
| C | 1.80206107 | 0.00000000 | -1.03389466 |
| N | -0.01743713 | 0.00000000 | 0.84742344 |
| N | -2.25203764 | 0.00000000 | 0.54034983 |
| H | 3.74280590 | 0.00000000 | -0.44375913 |
| H | 1.20115546 | 0.00000000 | -2.98380249 |

## S1.45 Difluorodiazirine

CASRN: 693-85-6 (Difluoro-3*H*-diazirine)

Level of theory: CC3(Full)/*aug*-cc-pVTZ

| | | | |
|---|---|---|---|
| C | 0.00000000 | 0.00000000 | -0.15283028 |
| F | 0.00000000 | 2.06077297 | -1.57706828 |
| F | 0.00000000 | -2.06077297 | -1.57706828 |
| N | 1.20382241 | 0.00000000 | 2.20566821 |
| N | -1.20382241 | 0.00000000 | 2.20566821 |

## S1.46 Dimethylaminobenzonitrile

CASRN: 1197-19-9 (4-(Dimethylamino)benzonitrile)

Level of theory: CCSD(T)(FC)/cc-pVTZ

Planar

| | | | |
|---|---|---|---|
| C | 0.00000000 | 0.00000000 | -1.96083197 |
| C | 2.27891314 | 0.00000000 | -0.58294740 |
| C | -2.27891314 | 0.00000000 | -0.58294740 |
| C | 0.00000000 | 0.00000000 | 3.37434994 |
| C | 2.26711046 | 0.00000000 | 2.02803761 |
| C | -2.26711046 | 0.00000000 | 2.02803761 |
| C | 0.00000000 | 0.00000000 | 6.06798788 |
| C | 2.36485177 | 0.00000000 | -5.90186899 |
| C | -2.36485177 | 0.00000000 | -5.90186899 |
| N | 0.00000000 | 0.00000000 | -4.53733249 |
| N | 0.00000000 | 0.00000000 | 8.26382999 |
| H | 4.06469412 | 0.00000000 | -1.55103579 |
| H | -4.06469412 | 0.00000000 | -1.55103579 |
| H | 4.03369195 | 0.00000000 | 3.04099978 |
| H | -4.03369195 | 0.00000000 | 3.04099978 |
| H | 1.96836611 | 0.00000000 | -7.91292844 |
| H | -1.96836611 | 0.00000000 | -7.91292844 |
| H | 3.49551175 | -1.67111709 | -5.47003452 |
| H | 3.49551175 | 1.67111709 | -5.47003452 |
| H | -3.49551175 | 1.67111709 | -5.47003452 |
| H | -3.49551175 | -1.67111709 | -5.47003452 |

Twisted

| | | | |
|---|---|---|---|
| C | 0.00000000 | 0.00000000 | -1.92629020 |
| C | 2.27225178 | 0.00000000 | -0.58317962 |
| C | -2.27225178 | 0.00000000 | -0.58317962 |
| C | 0.00000000 | 0.00000000 | 3.35560653 |
| C | 2.28330254 | 0.00000000 | 2.03752961 |
| C | -2.28330254 | 0.00000000 | 2.03752961 |
| C | 0.00000000 | 0.00000000 | 6.05799119 |
| C | 0.00000000 | 2.39191725 | -5.88267373 |
| C | 0.00000000 | -2.39191725 | -5.88267373 |
| N | 0.00000000 | 0.00000000 | -4.58434634 |
| N | 0.00000000 | 0.00000000 | 8.25212738 |
| H | 4.02777860 | 0.00000000 | -1.61674521 |
| H | -4.02777860 | 0.00000000 | -1.61674521 |
| H | 4.03804248 | 0.00000000 | 3.06961213 |
| H | -4.03804248 | 0.00000000 | 3.06961213 |
| H | 0.00000000 | 2.05258096 | -7.90903256 |
| H | 0.00000000 | -2.05258096 | -7.90903256 |
| H | 1.66857920 | 3.52919279 | -5.43615170 |

| | | | |
|---|---|---|---|
| H | -1.66857920 | 3.52919279 | -5.43615170 |
| H | -1.66857920 | -3.52919279 | -5.43615170 |
| H | 1.66857920 | -3.52919279 | -5.43615170 |

## S1.47 Dimethylaniline

CASRN: 121-69-7 (*N*,*N*-Dimethylaniline)

Level of theory: CCSD(T)(FC)/cc-pVTZ

| | | | |
|---|---|---|---|
| C | 0.00000000 | 0.00000000 | 4.89686867 |
| C | 2.25704297 | 0.00000000 | 3.55138467 |
| C | -2.25704297 | 0.00000000 | 3.55138467 |
| C | 2.27412639 | 0.00000000 | 0.92841898 |
| C | -2.27412639 | 0.00000000 | 0.92841898 |
| C | 0.00000000 | 0.00000000 | -0.44595239 |
| C | 2.36139267 | 0.00000000 | -4.39675011 |
| C | -2.36139267 | 0.00000000 | -4.39675011 |
| N | 0.00000000 | 0.00000000 | -3.03916783 |
| H | 4.05922248 | 0.00000000 | -0.04344476 |
| H | -4.05922248 | 0.00000000 | -0.04344476 |
| H | 4.03670718 | 0.00000000 | 4.54551891 |
| H | -4.03670718 | 0.00000000 | 4.54551891 |
| H | 0.00000000 | 0.00000000 | 6.93154996 |
| H | 1.97020408 | 0.00000000 | -6.40997108 |
| H | -1.97020408 | 0.00000000 | -6.40997108 |
| H | 3.49800498 | -1.66955347 | -3.96565000 |
| H | 3.49800498 | 1.66955347 | -3.96565000 |
| H | -3.49800498 | 1.66955347 | -3.96565000 |
| H | -3.49800498 | -1.66955347 | -3.96565000 |

## S1.48 Dinitrogen

CASRN: 7727-37-9

Level of theory: CC3(Full)/*aug*-cc-pVTZ

| | | | |
|---|---|---|---|
| N | 0.00000000 | 0.00000000 | 1.04008632 |
| N | 0.00000000 | 0.00000000 | -1.04008632 |

## S1.49 Ethylene

CASRN: 74-85-1

Level of theory: CC3(Full)/*aug*-cc-pVTZ

| | | | |
|---|---|---|---|
| C | 0.00000000 | 1.26026583 | 0.00000000 |
| C | 0.00000000 | -1.26026583 | 0.00000000 |
| H | 0.00000000 | 2.32345976 | 1.74287672 |
| H | 0.00000000 | -2.32345976 | 1.74287672 |
| H | 0.00000000 | 2.32345976 | -1.74287672 |
| H | 0.00000000 | -2.32345976 | -1.74287672 |

## S1.50 Fluorobenzene

CASRN: 462-06-6

Level of theory: CC3(FC)/cc-pVTZ

| | | | |
|---|---|---|---|
| F | 0.00000000 | 0.00000000 | -4.15873063 |
| C | 0.00000000 | 0.00000000 | -1.61842149 |
| C | 2.29188824 | 0.00000000 | -0.35805545 |
| C | -2.29188824 | 0.00000000 | -0.35805545 |
| C | 0.00000000 | 0.00000000 | 3.59063853 |
| C | 2.27621870 | 0.00000000 | 2.27153776 |
| C | -2.27621870 | 0.00000000 | 2.27153776 |
| H | 4.02397454 | 0.00000000 | -1.42355397 |
| H | -4.02397454 | 0.00000000 | -1.42355397 |
| H | 4.04329770 | 0.00000000 | 3.28356917 |
| H | -4.04329770 | 0.00000000 | 3.28356917 |
| H | 0.00000000 | 0.00000000 | 5.62589878 |

## S1.51 Formaldehyde

CASRN: 50-00-0

Level of theory: CC3(Full)/*aug*-cc-pVTZ

Ground state

| | | | |
|---|---|---|---|
| C | 0.00000000 | 0.00000000 | -1.13947666 |
| O | 0.00000000 | 0.00000000 | 1.14402883 |
| H | 0.00000000 | 1.76627623 | -2.23398653 |
| H | 0.00000000 | -1.76627623 | -2.23398653 |

Excited state

| | | | |
|---|---|---|---|
| C | -0.09942705 | 0.00000000 | 1.27071070 |
| O | 0.01987299 | 0.00000000 | -1.23280536 |
| H | 0.42778855 | 1.76729629 | 2.18470884 |
| H | 0.42778855 | -1.76729629 | 2.18470884 |

## S1.52 Formamide

CASRN: 75-12-7

Level of theory: CC3(Full)/*aug*-cc-pVTZ

| | | | |
|---|---|---|---|
| C | 0.00183118 | 0.00000000 | 0.79313299 |
| O | 2.26817156 | 0.00000000 | 0.43918824 |
| N | -1.76886033 | 0.00000000 | -1.06219243 |
| H | -0.84133459 | 0.00000000 | 2.68872485 |
| H | -1.21254414 | 0.00000000 | -2.87596907 |
| H | -3.61627502 | 0.00000000 | -0.65031317 |

## S1.53 Formylfluoride

CASRN: 1493-02-3 (Fomyl fluoride)

Level of theory: CC3(Full)/*aug*-cc-pVTZ

| | | | |
|---|---|---|---|
| C | 0.00536098 | 0.00000000 | 0.75320959 |
| O | 2.17369813 | 0.00000000 | 0.22287752 |
| H | -0.83846350 | 0.00000000 | 2.62640974 |
| F | -1.84051320 | 0.00000000 | -0.99373750 |

## S1.54 Furan

CASRN: 110-00-9

Level of theory: CC3(Full)/*aug*-cc-pVTZ

| | | | |
|---|---|---|---|
| C | 0.00000000 | 2.06365826 | -0.60051250 |
| C | 0.00000000 | -2.06365826 | -0.60051250 |
| C | 0.00000000 | 1.35348578 | 1.86336416 |
| C | 0.00000000 | -1.35348578 | 1.86336416 |
| O | 0.00000000 | 0.00000000 | -2.13945332 |
| H | 0.00000000 | 3.86337287 | -1.53765695 |
| H | 0.00000000 | -3.86337287 | -1.53765695 |
| H | 0.00000000 | 2.59168789 | 3.47168051 |
| H | 0.00000000 | -2.59168789 | 3.47168051 |

## S1.55 Furofuran

CASRN: 251-24-1 (Furo[3,2-*b*]furan)

Level of theory: CC3(FC)/cc-pVTZ

| | | | |
|---|---|---|---|
| C | 0.06548932 | 1.28240874 | 0.00000000 |
| C | -0.06548932 | -1.28240874 | 0.00000000 |
| C | -2.43794558 | 2.25427215 | 0.00000000 |
| C | 2.43794558 | -2.25427215 | 0.00000000 |
| C | -3.90023785 | 0.12403225 | 0.00000000 |
| C | 3.90023785 | -0.12403225 | 0.00000000 |
| O | 2.50066120 | 2.07485533 | 0.00000000 |
| O | -2.50066120 | -2.07485533 | 0.00000000 |
| H | -3.10620733 | 4.16541687 | 0.00000000 |
| H | 3.10620733 | -4.16541687 | 0.00000000 |
| H | -5.90761266 | -0.13384378 | 0.00000000 |
| H | 5.90761266 | 0.13384378 | 0.00000000 |

## S1.56 Glyoxal

CASRN: 107-22-2

Level of theory: CC3(Full)/*aug*-cc-pVTZ

| | | | |
|---|---|---|---|
| C | 1.21360282 | 0.75840215 | 0.00000000 |
| C | -1.21360282 | -0.75840215 | 0.00000000 |
| O | 3.25581408 | -0.26453186 | 0.00000000 |
| O | -3.25581408 | 0.26453186 | 0.00000000 |
| H | 0.96135276 | 2.81883243 | 0.00000000 |
| H | -0.96135276 | -2.81883243 | 0.00000000 |

## S1.57 HCCl

CASRN: 2108-20-5 (Chlorocarbene)

Level of theory: CC3(Full)/*aug*-cc-pVTZ

| | | | |
|---|---|---|---|
| H | -1.88068369 | 0.00000000 | -0.14323924 |
| Cl | 2.28559426 | 0.00000000 | -0.43261163 |
| C | -0.40491057 | 0.00000000 | 1.32161964 |

## S1.58 HCF

CASRN: 13453-52-6 (Fluorocarbene)

Level of theory: CC3(Full)/*aug*-cc-pVTZ

| | | | |
|---|---|---|---|
| C | -0.13561085 | 0.00000000 | 1.20394474 |
| F | 1.85493976 | 0.00000000 | -0.27610752 |
| H | -1.71932891 | 0.00000000 | -0.18206846 |

## S1.59 HCN

CASRN: 74-90-8 (Hydrogen cyanide)

Level of theory: CC3(FC)/*aug*-cc-pVTZ

| | | | |
|---|---|---|---|
| H | 0.00000000 | 0.00000000 | 3.06256364 |
| C | 0.00000000 | 0.00000000 | 1.05824145 |
| N | 0.00000000 | 0.00000000 | -1.12728289 |

## S1.60 HCP

CASRN: 6829-52-3 (Phosphine, methylidyne-)

Level of theory: CC3(Full)/*aug*-cc-pVTZ

| | | | |
|---|---|---|---|
| H | 0.00000000 | 0.00000000 | -4.03090449 |
| C | 0.00000000 | 0.00000000 | -2.01691641 |
| P | 0.00000000 | 0.00000000 | 0.91401621 |

## S1.61 Hexatriene

CASRN: 2235-12-3

Level of theory: CC3(Full)/*aug*-cc-pVTZ

| | | | |
|---|---|---|---|
| C | 1.14024826 | 0.56596845 | 0.00000000 |
| C | -1.14024826 | -0.56596845 | 0.00000000 |
| C | 3.51540649 | -0.78907931 | 0.00000000 |
| C | -3.51540649 | 0.78907931 | 0.00000000 |
| C | 5.78668151 | 0.33754155 | 0.00000000 |
| C | -5.78668151 | -0.33754155 | 0.00000000 |
| H | 1.23448067 | 2.61584039 | 0.00000000 |

| | | | |
|---|---|---|---|
| H | -1.23448067 | -2.61584039 | 0.00000000 |
| H | 3.40773630 | -2.83459321 | 0.00000000 |
| H | -3.40773630 | 2.83459321 | 0.00000000 |
| H | 5.95047109 | 2.37626316 | 0.00000000 |
| H | -5.95047109 | -2.37626316 | 0.00000000 |
| H | 7.51470672 | -0.74809921 | 0.00000000 |
| H | -7.51470672 | 0.74809921 | 0.00000000 |

## S1.62 HNC

CASRN: 6914-07-4 (Hydrogen isocyanide)

Level of theory: CC3(FC)/*aug*-cc-pVTZ

| | | | |
|---|---|---|---|
| H | 0.00000000 | 0.00000000 | 2.79539858 |
| N | 0.00000000 | 0.00000000 | 0.91469554 |
| C | 0.00000000 | 0.00000000 | -1.30215184 |

## S1.63 HPO

CASRN: 13817-06-6 (Oxophosphine)

Level of theory: CC3(Full)/*aug*-cc-pVTZ

| | | | |
|---|---|---|---|
| H | 0.31668637 | 0.00000000 | 0.14072725 |
| P | -0.80573521 | 0.00000000 | 2.65136926 |
| O | 1.43391190 | 0.00000000 | 4.38886277 |

## S1.64 HPS

CASRN: 109306-51-6 (Thioxophosphine)

Level of theory: CC3(Full)/*aug*-cc-pVTZ

| | | | |
|---|---|---|---|
| H | -2.56278959 | 0.00000000 | 2.36296006 |
| P | 0.09114182 | 0.00000000 | 1.82568543 |
| S | 0.07946992 | 0.00000000 | -1.85778170 |

## S1.65 HSiF

CASRN: 50561-30-3 (Fluorosilylene)

Level of theory: CC3(Full)/*aug*-cc-pVTZ

| | | | |
|---|---|---|---|
| Si | -0.06438136 | 0.00000000 | 1.67253150 |
| F | 2.24990164 | 0.00000000 | -0.33928119 |
| H | -2.18552027 | 0.00000000 | -0.28748154 |

## S1.66 Hydrogen chloride

CASRN: 7647-01-0

Level of theory: CC3(Full)/*aug*-cc-pVTZ

| | | | |
|---|---|---|---|
| Cl | 0.00000000 | 0.00000000 | -0.02489783 |
| H | 0.00000000 | 0.00000000 | 2.38483140 |

## S1.67 Hydrogen peroxide

CASRN: 7722-84-1

Level of theory: CC3(FC)/*aug*-cc-pVTZ

| | | | |
|---|---|---|---|
| O | -1.37083247 | -0.11183297 | -0.05928025 |
| O | 1.37083247 | 0.11183297 | -0.05928025 |
| H | -1.80587866 | 1.34729428 | 0.94082062 |
| H | 1.80587866 | -1.34729428 | 0.94082062 |

## S1.68 Hydrogen sulfide

CASRN: 7783-06-4

Level of theory: CC3(Full)/*aug*-cc-pVTZ

| | | | |
|---|---|---|---|
| S | 0.00000000 | 0.00000000 | -0.50365086 |
| H | 0.00000000 | 1.81828105 | 1.25212288 |
| H | 0.00000000 | -1.81828105 | 1.25212288 |

## S1.69 Imidazole

CASRN: 288-32-4

Level of theory: CC3(Full)/*aug*-cc-pVTZ

| | | | |
|---|---|---|---|
| C | 0.41662795 | 2.06006259 | 0.00000000 |
| C | -1.52618386 | -1.62343163 | 0.00000000 |
| C | 1.04160471 | -1.93007427 | 0.00000000 |
| N | -1.90345764 | 0.94914956 | 0.00000000 |
| N | 2.24215443 | 0.38083431 | 0.00000000 |
| H | 0.65501634 | 4.07748278 | 0.00000000 |
| H | -3.57500545 | 1.84103166 | 0.00000000 |
| H | -3.06363894 | -2.94559167 | 0.00000000 |
| H | 2.08673940 | -3.67001102 | 0.00000000 |

## S1.70 Isobutene

CASRN: 115-11-7

Level of theory: CC3(Full)/*aug*-cc-pVTZ

| | | | |
|---|---|---|---|
| C | 0.00000000 | 0.00000000 | 2.70790758 |
| C | 0.00000000 | 0.00000000 | 0.18431282 |
| C | 0.00000000 | 2.39894572 | -1.32482735 |
| C | 0.00000000 | -2.39894572 | -1.32482735 |
| H | 0.00000000 | 1.74848405 | 3.76691310 |
| H | 0.00000000 | -1.74848405 | 3.76691310 |
| H | 0.00000000 | 4.05897160 | -0.10582007 |
| H | 0.00000000 | -4.05897160 | -0.10582007 |
| H | 1.66026992 | 2.48337908 | -2.55086178 |
| H | -1.66026992 | 2.48337908 | -2.55086178 |
| H | 1.66026992 | -2.48337908 | -2.55086178 |
| H | -1.66026992 | -2.48337908 | -2.55086178 |

## S1.71 Ketene

CASRN: 463-51-4 (Ethenone)

Level of theory: CC3(Full)/*aug*-cc-pVTZ

Ground state

| | | | |
|---|---|---|---|
| C | 0.00000000 | 0.00000000 | -2.44810151 |
| C | 0.00000000 | 0.00000000 | 0.03498545 |
| O | 0.00000000 | 0.00000000 | 2.23663914 |
| H | 0.00000000 | 1.77432079 | -3.43705988 |
| H | 0.00000000 | -1.77432079 | -3.43705988 |

Excited state

| | | | |
|---|---|---|---|
| C | 2.04306304 | 0.00000000 | -0.93056721 |
| C | 0.00400918 | 0.00000000 | 0.83531393 |
| O | -2.23710378 | 0.00000000 | 0.46984584 |
| H | 1.63603518 | 0.00000000 | -2.93687368 |
| H | 3.96212800 | 0.00000000 | -0.26649149 |

## S1.72 Maleimide

CASRN: 541-59-3 (1*H*-Pyrrole-2,5-dione)

Level of theory: CC3(Full)/*aug*-cc-pVTZ

| | | | |
|---|---|---|---|
| C | 0.00000000 | 2.17350401 | 0.25165554 |
| C | 0.00000000 | -2.17350401 | 0.25165554 |
| C | 0.00000000 | 1.26218315 | -2.42188951 |
| C | 0.00000000 | -1.26218315 | -2.42188951 |
| N | 0.00000000 | 0.00000000 | 1.72344743 |
| O | 0.00000000 | 4.32709218 | 1.01147397 |
| O | 0.00000000 | -4.32709218 | 1.01147397 |
| H | 0.00000000 | 0.00000000 | 3.62206099 |
| H | 0.00000000 | 2.54941470 | -3.99634348 |
| H | 0.00000000 | -2.54941470 | -3.99634348 |

## S1.73 Methanimine

CASRN: 2053-29-4 (Formaldimine)

Level of theory: CC3(Full)/*aug*-cc-pVTZ

| | | | |
|---|---|---|---|
| C | 0.10696646 | 0.00000000 | 1.11091130 |
| N | 0.10764012 | 0.00000000 | -1.29677742 |
| H | -1.59140953 | 0.00000000 | 2.27296652 |
| H | 1.90475160 | 0.00000000 | 2.09393982 |
| H | -1.69956184 | 0.00000000 | -1.96217482 |

## S1.74 Methylenecyclopropene

CASRN: 4095-06-1

Level of theory: CC3(Full)/*aug*-cc-pVTZ

| | | | |
|---|---|---|---|
| C | 0.00000000 | 0.00000000 | 0.53512883 |
| C | 0.00000000 | 0.00000000 | 3.04739824 |

| | | | |
|---|---|---|---|
| C | 0.00000000 | 1.25042956 | -1.88571561 |
| C | 0.00000000 | -1.25042956 | -1.88571561 |
| H | 0.00000000 | 2.96887531 | -2.96270271 |
| H | 0.00000000 | -2.96887531 | -2.96270271 |
| H | 0.00000000 | 1.75335023 | 4.08608382 |
| H | 0.00000000 | -1.75335023 | 4.08608382 |

## S1.75 Naphthalene

CASRN: 91-20-3

Level of theory: CC3(Full)/cc-pVTZ

| | | | |
|---|---|---|---|
| C | 0.00000000 | 1.33999524 | 0.00000000 |
| C | 0.00000000 | -1.33999524 | 0.00000000 |
| C | 2.33779858 | 2.63841577 | 0.00000000 |
| C | -2.33779858 | 2.63841577 | 0.00000000 |
| C | 2.33779858 | -2.63841577 | 0.00000000 |
| C | -2.33779858 | -2.63841577 | 0.00000000 |
| C | 4.57964958 | 1.33587048 | 0.00000000 |
| C | -4.57964958 | 1.33587048 | 0.00000000 |
| C | 4.57964958 | -1.33587048 | 0.00000000 |
| C | -4.57964958 | -1.33587048 | 0.00000000 |
| H | 2.32888235 | 4.67949410 | 0.00000000 |
| H | -2.32888235 | 4.67949410 | 0.00000000 |
| H | 2.32888235 | -4.67949410 | 0.00000000 |
| H | -2.32888235 | -4.67949410 | 0.00000000 |
| H | 6.34884007 | 2.34551705 | 0.00000000 |
| H | -6.34884007 | 2.34551705 | 0.00000000 |
| H | 6.34884007 | -2.34551705 | 0.00000000 |
| H | -6.34884007 | -2.34551705 | 0.00000000 |

## S1.76 Nitroaniline

CASRN: 100-01-6 (4-Nitroaniline)

Level of theory: CC3(FC)/cc-pVTZ

| | | | |
|---|---|---|---|
| C | 0.00000000 | 0.00000000 | -4.05915738 |
| C | 2.28068352 | 0.00000000 | -2.70811066 |
| C | -2.28068352 | 0.00000000 | -2.70811066 |
| C | 0.00000000 | 0.00000000 | 1.19144079 |
| C | 2.28308329 | 0.00000000 | -0.09681843 |

| | | | |
|---|---|---|---|
| C | -2.28308329 | 0.00000000 | -0.09681843 |
| N | 0.00000000 | 0.00000000 | 3.94052757 |
| N | 0.00000000 | 0.00000000 | -6.63741535 |
| O | 2.04948184 | 0.00000000 | 5.01410797 |
| O | -2.04948184 | 0.00000000 | 5.01410797 |
| H | 4.04799128 | 0.00000000 | -3.72195018 |
| H | -4.04799128 | 0.00000000 | -3.72195018 |
| H | 4.02032559 | 0.00000000 | 0.95557275 |
| H | -4.02032559 | 0.00000000 | 0.95557275 |
| H | -1.62132329 | 0.00000000 | -7.60488781 |
| H | 1.62132329 | 0.00000000 | -7.60488781 |

## S1.77 Nitrobenzene

CASRN: 98-95-3

Level of theory: CC3(FC)/cc-pVTZ

| | | | |
|---|---|---|---|
| C | 0.00000000 | 0.00000000 | -0.33719774 |
| C | 2.29667056 | 0.00000000 | 0.92138137 |
| C | -2.29667056 | 0.00000000 | 0.92138137 |
| C | 0.00000000 | 0.00000000 | 4.85826496 |
| C | 2.28247086 | 0.00000000 | 3.54756893 |
| C | -2.28247086 | 0.00000000 | 3.54756893 |
| N | 0.00000000 | 0.00000000 | -3.11429157 |
| O | -2.05476165 | 0.00000000 | -4.18095202 |
| O | 2.05476165 | 0.00000000 | -4.18095202 |
| H | 4.02347357 | 0.00000000 | -0.14769848 |
| H | -4.02347357 | 0.00000000 | -0.14769848 |
| H | 4.04624818 | 0.00000000 | 4.56388578 |
| H | -4.04624818 | 0.00000000 | 4.56388578 |
| H | 0.00000000 | 0.00000000 | 6.89454456 |

## S1.78 Nitrodimethylaniniline

CASRN: 100-23-2 (*N*,*N*-Dimethyl-4-nitroaniline)

Level of theory: CCSD(T)(FC)/cc-pVTZ

| | | | |
|---|---|---|---|
| C | 0.00000000 | 0.00000000 | -2.70893747 |
| C | 2.28286889 | 0.00000000 | -1.33300281 |
| C | -2.28286889 | 0.00000000 | -1.33300281 |
| C | 0.00000000 | 0.00000000 | 2.57206374 |

| | | | |
|---|---|---|---|
| C | 2.27821428 | 0.00000000 | 1.27798588 |
| C | -2.27821428 | 0.00000000 | 1.27798588 |
| C | 2.36504204 | 0.00000000 | -6.64945038 |
| C | -2.36504204 | 0.00000000 | -6.64945038 |
| N | 0.00000000 | 0.00000000 | -5.28314977 |
| N | 0.00000000 | 0.00000000 | 5.31851989 |
| O | 2.04957627 | 0.00000000 | 6.39360902 |
| O | -2.04957627 | 0.00000000 | 6.39360902 |
| H | 4.06683325 | 0.00000000 | -2.30372191 |
| H | -4.06683325 | 0.00000000 | -2.30372191 |
| H | 4.01906768 | 0.00000000 | 2.32551175 |
| H | -4.01906768 | 0.00000000 | 2.32551175 |
| H | 1.96723800 | 0.00000000 | -8.66013185 |
| H | -1.96723800 | 0.00000000 | -8.66013185 |
| H | 3.49498309 | -1.67118066 | -6.21739275 |
| H | 3.49498309 | 1.67118066 | -6.21739275 |
| H | -3.49498309 | 1.67118066 | -6.21739275 |
| H | -3.49498309 | -1.67118066 | -6.21739275 |

## S1.79 Nitropyridine *N*-oxide

CASRN: 1124-33-0 (4-Nitropyridine *N*-oxide)

Level of theory: CCSD(T)(FC)/cc-pVTZ

| | | | |
|---|---|---|---|
| C | 0.00000000 | 0.00000000 | -1.21738204 |
| C | 2.26825255 | 0.00000000 | 0.09038008 |
| C | -2.26825255 | 0.00000000 | 0.09038008 |
| C | 2.22988276 | 0.00000000 | 2.68605086 |
| C | -2.22988276 | 0.00000000 | 2.68605086 |
| N | 0.00000000 | 0.00000000 | -3.96704616 |
| N | 0.00000000 | 0.00000000 | 4.00601244 |
| O | 0.00000000 | 0.00000000 | 6.38961931 |
| O | -2.05398155 | 0.00000000 | -5.02438491 |
| O | 2.05398155 | 0.00000000 | -5.02438491 |
| H | 4.03491913 | 0.00000000 | -0.90939267 |
| H | -4.03491913 | 0.00000000 | -0.90939267 |
| H | 3.88274506 | 0.00000000 | 3.86446617 |
| H | -3.88274506 | 0.00000000 | 3.86446617 |

## S1.80 Nitrosomethane

CASRN: 865-40-7

Level of theory: CC3(Full)/*aug*-cc-pVTZ

Ground state

| | | | |
|---|---|---|---|
| C | -1.78426612 | 0.00000000 | -1.07224050 |
| N | -0.00541753 | 0.00000000 | 1.08060391 |
| O | 2.18814985 | 0.00000000 | 0.43452135 |
| H | -0.77343975 | 0.00000000 | -2.86415606 |
| H | -2.97471478 | 1.66801808 | -0.86424584 |
| H | -2.97471478 | -1.66801808 | -0.86424584 |

Excited state

| | | | |
|---|---|---|---|
| C | 1.86306273 | 0.00000000 | -1.06035094 |
| N | 0.00638693 | 0.00000000 | 1.02546010 |
| O | -2.26923072 | 0.00000000 | 0.47699489 |
| H | 3.72600129 | 0.00000000 | -0.21094854 |
| H | 1.58491147 | 1.68964774 | -2.20977225 |
| H | 1.58491147 | -1.68964774 | -2.20977225 |

## S1.81 Nitrous acid

CASRN: 7782-77-6

Level of theory: CC3(FC)/*aug*-cc-pVTZ

| | | | |
|---|---|---|---|
| H | -3.27788005 | 0.93588010 | 0.00000000 |
| N | 0.29308547 | 0.93895729 | 0.00000000 |
| O | -2.05678600 | -0.42335161 | 0.00000000 |
| O | 2.00673459 | -0.45764664 | 0.00000000 |

## S1.82 Nitrous oxide

CASRN: 10024-97-2

Level of theory: CC3(FC)/*aug*-cc-pVTZ

| | | | |
|---|---|---|---|
| N | 0.00000000 | 0.00000000 | 0.13652607 |
| N | 0.00000000 | 0.00000000 | 2.27480281 |
| O | 0.00000000 | 0.00000000 | -2.11104702 |

## S1.83 Nitroxyl

CASRN: 14332-28-6

Level of theory: CC3(Full)/*aug*-cc-pVTZ

| | | | |
|---|---|---|---|
| O | 0.21099695 | 0.00000000 | 2.15462460 |
| N | -0.44776863 | 0.00000000 | -0.03589263 |
| H | 1.18163475 | 0.00000000 | -1.17386890 |

## S1.84 Octatetraene

CASRN: 1482-91-3

Level of theory: CC3(Full)/cc-pVTZ

| | | | |
|---|---|---|---|
| C | 1.19649232 | 0.64794934 | 0.00000000 |
| C | -1.19649232 | -0.64794934 | 0.00000000 |
| C | 3.45745137 | -0.52964709 | 0.00000000 |
| C | -3.45745137 | 0.52964709 | 0.00000000 |
| C | 5.85705040 | 0.77625595 | 0.00000000 |
| C | -5.85705040 | -0.77625595 | 0.00000000 |
| C | 8.10525884 | -0.39700663 | 0.00000000 |
| C | -8.10525884 | 0.39700663 | 0.00000000 |
| H | 1.14813002 | 2.69304901 | 0.00000000 |
| H | -1.14813002 | -2.69304901 | 0.00000000 |
| H | 3.50962357 | -2.57436634 | 0.00000000 |
| H | -3.50962357 | 2.57436634 | 0.00000000 |
| H | 5.78969253 | 2.81832245 | 0.00000000 |
| H | -5.78969253 | -2.81832245 | 0.00000000 |
| H | 8.22516217 | -2.43500100 | 0.00000000 |
| H | -8.22516217 | 2.43500100 | 0.00000000 |
| H | 9.85247043 | 0.65022932 | 0.00000000 |
| H | -9.85247043 | -0.65022932 | 0.00000000 |

## S1.85 Oxalyl fluoride

CASRN: 359-40-0

Level of theory: CC3(Full)/*aug*-cc-pVTZ

| | | | |
|---|---|---|---|
| C | -1.39903565 | 0.34476183 | 0.00000000 |
| C | 1.39903565 | -0.34476183 | 0.00000000 |
| O | -2.24825627 | 2.40855549 | 0.00000000 |

| | | | |
|---|---|---|---|
| O | 2.24825627 | -2.40855549 | 0.00000000 |
| F | -2.78737061 | -1.74488227 | 0.00000000 |
| F | 2.78737061 | 1.74488227 | 0.00000000 |

## S1.86 Pentalene

CASRN: 250-25-9

Level of theory: CC3(FC)/cc-pVTZ

| | | | |
|---|---|---|---|
| C | -0.07378347 | 1.37547375 | 0.00000000 |
| C | 0.07378347 | -1.37547375 | 0.00000000 |
| C | 2.30364735 | 2.30974227 | 0.00000000 |
| C | -2.30364735 | -2.30974227 | 0.00000000 |
| C | 4.08788978 | 0.11767244 | 0.00000000 |
| C | -4.08788978 | -0.11767244 | 0.00000000 |
| C | 2.75907835 | -2.07144063 | 0.00000000 |
| C | -2.75907835 | 2.07144063 | 0.00000000 |
| H | 2.88453811 | 4.25947081 | 0.00000000 |
| H | -2.88453811 | -4.25947081 | 0.00000000 |
| H | 6.11180520 | 0.29622071 | 0.00000000 |
| H | -6.11180520 | -0.29622071 | 0.00000000 |
| H | 3.52044397 | -3.95397547 | 0.00000000 |
| H | -3.52044397 | 3.95397547 | 0.00000000 |

Level of theory: CC3(FC)/cc-pVTZ [$D_{2h}$ constrained]

| | | | |
|---|---|---|---|
| C | 0.00000000 | -1.32183553 | 0.00000000 |
| C | 4.12643396 | 0.00000000 | 0.00000000 |
| C | 0.00000000 | 1.32183553 | 0.00000000 |
| C | -4.12643396 | 0.00000000 | 0.00000000 |
| C | 2.55477535 | -2.15447186 | 0.00000000 |
| C | -2.55477535 | -2.15447186 | 0.00000000 |
| C | 2.55477535 | 2.15447186 | 0.00000000 |
| C | -2.55477535 | 2.15447186 | 0.00000000 |
| H | 6.15419256 | 0.00000000 | 0.00000000 |
| H | -6.15419256 | 0.00000000 | 0.00000000 |
| H | 3.20834414 | -4.08294363 | 0.00000000 |
| H | -3.20834414 | -4.08294363 | 0.00000000 |
| H | 3.20834414 | 4.08294363 | 0.00000000 |
| H | -3.20834414 | 4.08294363 | 0.00000000 |

## S1.87 Phenol

CASRN: 108-95-2

Level of theory: CC3(FC)/cc-pVTZ

| | | | |
|---|---|---|---|
| C | -3.53896151 | -0.00090430 | 0.00000000 |
| C | -2.20193059 | -2.26940360 | 0.00000000 |
| C | 0.42215955 | -2.27848829 | 0.00000000 |
| C | 1.72887083 | 0.00401463 | 0.00000000 |
| C | 0.41326561 | 2.28038150 | 0.00000000 |
| C | -2.21662249 | 2.26943538 | 0.00000000 |
| O | 4.30714712 | -0.10549070 | 0.00000000 |
| H | -5.57402535 | -0.00548883 | 0.00000000 |
| H | -3.20490358 | -4.04260115 | 0.00000000 |
| H | 1.47915023 | -4.01756951 | 0.00000000 |
| H | 1.43787439 | 4.04468538 | 0.00000000 |
| H | -3.22333595 | 4.04049312 | 0.00000000 |
| H | 4.94381975 | 1.59474054 | 0.00000000 |

## S1.88 Phenolate

CASRN: 3229-70-7

Level of theory: CC3(FC)/cc-pVTZ

| | | | |
|---|---|---|---|
| C | 0.00000000 | 0.00000000 | -1.94817868 |
| C | 2.27737723 | 0.00000000 | -0.45104645 |
| C | -2.27737723 | 0.00000000 | -0.45104645 |
| C | 0.00000000 | 0.00000000 | 3.54287236 |
| C | 2.25856599 | 0.00000000 | 2.16672471 |
| C | -2.25856599 | 0.00000000 | 2.16672471 |
| O | 0.00000000 | 0.00000000 | -4.33677175 |
| H | 4.04811102 | 0.00000000 | -1.47084405 |
| H | -4.04811102 | 0.00000000 | -1.47084405 |
| H | 4.04319440 | 0.00000000 | 3.17158878 |
| H | -4.04319440 | 0.00000000 | 3.17158878 |
| H | 0.00000000 | 0.00000000 | 5.58190673 |

## S1.89 Phenyl-pyrrole

CASRN: 635-90-5 (*N*-Phenylpyrrole)

Level of theory: CCSD(T)(FC)/cc-pVTZ

Planar

| | | | |
|---|---|---|---|
| C | 0.00000000 | 0.00000000 | 0.78511855 |
| C | 2.26951425 | 0.00000000 | 2.12513335 |
| C | -2.26951425 | 0.00000000 | 2.12513335 |
| C | 0.00000000 | 0.00000000 | 6.08505036 |
| C | 2.26188550 | 0.00000000 | 4.74952804 |
| C | -2.26188550 | 0.00000000 | 4.74952804 |
| C | 2.11189435 | 0.00000000 | -3.40622062 |
| C | -2.11189435 | 0.00000000 | -3.40622062 |
| C | 1.34457992 | 0.00000000 | -5.87759851 |
| C | -1.34457992 | 0.00000000 | -5.87759851 |
| N | 0.00000000 | 0.00000000 | -1.87596109 |
| H | 4.04529764 | 0.00000000 | 1.13844406 |
| H | -4.04529764 | 0.00000000 | 1.13844406 |
| H | 4.03918748 | 0.00000000 | 5.74456463 |
| H | -4.03918748 | 0.00000000 | 5.74456463 |
| H | 0.00000000 | 0.00000000 | 8.12006610 |
| H | 3.97993856 | 0.00000000 | -2.63372956 |
| H | -3.97993856 | 0.00000000 | -2.63372956 |
| H | 2.56993408 | 0.00000000 | -7.49221560 |
| H | -2.56993408 | 0.00000000 | -7.49221560 |

Twisted

| | | | |
|---|---|---|---|
| C | 0.00000000 | 0.00000000 | 0.80351712 |
| C | 2.28073444 | 0.00000000 | 2.10816686 |
| C | -2.28073444 | 0.00000000 | 2.10816686 |
| C | 0.00000000 | 0.00000000 | 6.05091031 |
| C | 2.27731959 | 0.00000000 | 4.73583348 |
| C | -2.27731959 | 0.00000000 | 4.73583348 |
| C | 0.00000000 | 2.11496090 | -3.38187966 |
| C | 0.00000000 | -2.11496090 | -3.38187966 |
| C | 0.00000000 | 1.34265418 | -5.86240596 |
| C | 0.00000000 | -1.34265418 | -5.86240596 |
| N | 0.00000000 | 0.00000000 | -1.87814812 |
| H | 4.02558097 | 0.00000000 | 1.05801658 |
| H | -4.02558097 | 0.00000000 | 1.05801658 |
| H | 4.04316226 | 0.00000000 | 5.75023395 |
| H | -4.04316226 | 0.00000000 | 5.75023395 |
| H | 0.00000000 | 0.00000000 | 8.08702673 |
| H | 0.00000000 | 3.96297102 | -2.54995976 |
| H | 0.00000000 | -3.96297102 | -2.54995976 |
| H | 0.00000000 | 2.56243264 | -7.48144109 |
| H | 0.00000000 | -2.56243264 | -7.48144109 |

## S1.90 Phthalazine

CASRN: 253-52-1

Level of theory: CC3(FC)/cc-pVTZ

| | | | |
|---|---|---|---|
| C | 0.00000000 | 1.32459443 | -0.07132677 |
| C | 0.00000000 | -1.32459443 | -0.07132677 |
| C | 0.00000000 | 2.65486490 | -2.37693013 |
| C | 0.00000000 | -2.65486490 | -2.37693013 |
| C | 0.00000000 | 1.33510515 | -4.61541123 |
| C | 0.00000000 | -1.33510515 | -4.61541123 |
| C | 0.00000000 | 2.49806192 | 2.33813333 |
| C | 0.00000000 | -2.49806192 | 2.33813333 |
| N | 0.00000000 | 1.29575320 | 4.50170701 |
| N | 0.00000000 | -1.29575320 | 4.50170701 |
| H | 0.00000000 | 4.69409431 | -2.36246981 |
| H | 0.00000000 | -4.69409431 | -2.36246981 |
| H | 0.00000000 | 2.33538579 | -6.38945264 |
| H | 0.00000000 | -2.33538579 | -6.38945264 |
| H | 0.00000000 | 4.53863166 | 2.46976178 |
| H | 0.00000000 | -4.53863166 | 2.46976178 |

## S1.91 Propynal

CASRN: 624-67-9

Level of theory: CC3(Full)/*aug*-cc-pVTZ

| | | | |
|---|---|---|---|
| C | -0.78051115 | 0.00000000 | -1.38900384 |
| C | -0.17873562 | 0.00000000 | 1.27825868 |
| C | 0.23763714 | 0.00000000 | 3.52644798 |
| O | 0.80143996 | 0.00000000 | -3.04628328 |
| H | -2.80713069 | 0.00000000 | -1.82768750 |
| H | 0.64026209 | 0.00000000 | 5.48853193 |

## S1.92 Pyranone

CASRN: 108-97-4 (4*H*-Pyran-4-one)

Level of theory: CC3(FC)/cc-pVTZ

| | | | |
|---|---|---|---|
| C | 0.00000000 | 0.00000000 | -2.03875103 |
| C | 2.29857501 | 0.00000000 | -0.50612872 |

| | | | |
|---|---|---|---|
| C | -2.29857501 | 0.00000000 | -0.50612872 |
| C | 2.18356567 | 0.00000000 | 2.02781371 |
| C | -2.18356567 | 0.00000000 | 2.02781371 |
| O | 0.00000000 | 0.00000000 | 3.36810442 |
| O | 0.00000000 | 0.00000000 | -4.35224344 |
| H | 3.80117763 | 0.00000000 | 3.26042029 |
| H | -3.80117763 | 0.00000000 | 3.26042029 |
| H | 4.10758504 | 0.00000000 | -1.43183287 |
| H | -4.10758504 | 0.00000000 | -1.43183287 |

## S1.93 Pyrazine

CASRN: 290-37-9

Level of theory: CC3(Full)/*aug*-cc-pVTZ

| | | | |
|---|---|---|---|
| C | 0.00000000 | 2.13188686 | 1.31510863 |
| C | 0.00000000 | -2.13188686 | 1.31510863 |
| C | 0.00000000 | 2.13188686 | -1.31510863 |
| C | 0.00000000 | -2.13188686 | -1.31510863 |
| N | 0.00000000 | 0.00000000 | 2.66620111 |
| N | 0.00000000 | 0.00000000 | -2.66620111 |
| H | 0.00000000 | 3.88751412 | 2.35234226 |
| H | 0.00000000 | -3.88751412 | 2.35234226 |
| H | 0.00000000 | 3.88751412 | -2.35234226 |
| H | 0.00000000 | -3.88751412 | -2.35234226 |

## S1.94 Pyridazine

CASRN: 289-80-5

Level of theory: CC3(Full)/*aug*-cc-pVTZ

| | | | |
|---|---|---|---|
| C | 0.00000000 | 1.30150855 | -2.31552865 |
| C | 0.00000000 | -1.30150855 | -2.31552865 |
| C | 0.00000000 | 2.49271907 | 0.03513416 |
| C | 0.00000000 | -2.49271907 | 0.03513416 |
| N | 0.00000000 | 1.26228251 | 2.23104685 |
| N | 0.00000000 | -1.26228251 | 2.23104685 |
| H | 0.00000000 | 4.52804172 | 0.19299731 |
| H | 0.00000000 | -4.52804172 | 0.19299731 |
| H | 0.00000000 | 2.39011496 | -4.03967703 |
| H | 0.00000000 | -2.39011496 | -4.03967703 |

## S1.95 Pyridine

CASRN: 110-86-1

Level of theory: CC3(Full)/*aug*-cc-pVTZ

| | | | |
|---|---|---|---|
| C | 0.00000000 | 0.00000000 | -2.66451139 |
| C | 0.00000000 | 2.25494985 | -1.32069889 |
| C | 0.00000000 | -2.25494985 | -1.32069889 |
| C | 0.00000000 | 2.15398594 | 1.30669632 |
| C | 0.00000000 | -2.15398594 | 1.30669632 |
| N | 0.00000000 | 0.00000000 | 2.62778932 |
| H | 0.00000000 | 0.00000000 | -4.70641516 |
| H | 0.00000000 | 4.05768507 | -2.27625442 |
| H | 0.00000000 | -4.05768507 | -2.27625442 |
| H | 0.00000000 | 3.88059079 | 2.40341581 |
| H | 0.00000000 | -3.88059079 | 2.40341581 |

## S1.96 Pyridinium

CASRN: 16969-45-2

Level of theory: CC3(FC)/cc-pVTZ

| | | | |
|---|---|---|---|
| C | 0.00000000 | 0.00000000 | -2.66667191 |
| C | 2.28175579 | 0.00000000 | -1.35203950 |
| C | -2.28175579 | 0.00000000 | -1.35203950 |
| C | 2.23916852 | 0.00000000 | 1.25404098 |
| C | -2.23916852 | 0.00000000 | 1.25404098 |
| N | 0.00000000 | 0.00000000 | 2.46287949 |
| H | 0.00000000 | 0.00000000 | -4.70272202 |
| H | 4.06725168 | 0.00000000 | -2.32197291 |
| H | -4.06725168 | 0.00000000 | -2.32197291 |
| H | 3.90684584 | 0.00000000 | 2.41825457 |
| H | -3.90684584 | 0.00000000 | 2.41825457 |
| H | 0.00000000 | 0.00000000 | 4.37535718 |

## S1.97 Pyrimidine

CASRN: 289-95-2

Level of theory: CC3(Full)/*aug*-cc-pVTZ

| | | | |
|---|---|---|---|
| C | 0.00000000 | 0.00000000 | 2.41518350 |
| C | 0.00000000 | 0.00000000 | -2.60410885 |
| C | 0.00000000 | 2.23272561 | -1.22869402 |
| C | 0.00000000 | -2.23272561 | -1.22869402 |
| N | 0.00000000 | 2.26214196 | 1.29619742 |
| N | 0.00000000 | -2.26214196 | 1.29619742 |
| H | 0.00000000 | 0.00000000 | 4.45780256 |
| H | 0.00000000 | 0.00000000 | -4.64120942 |
| H | 0.00000000 | 4.05149341 | -2.16351748 |
| H | 0.00000000 | -4.05149341 | -2.16351748 |

## S1.98 Pyrrole

CASRN: 109-97-7

Level of theory: CC3(Full)/*aug*-cc-pVTZ

| | | | |
|---|---|---|---|
| C | 0.00000000 | 2.11924634 | 0.62676569 |
| C | 0.00000000 | -2.11924634 | 0.62676569 |
| C | 0.00000000 | 1.34568862 | -1.85506908 |
| C | 0.00000000 | -1.34568862 | -1.85506908 |
| N | 0.00000000 | 0.00000000 | 2.10934391 |
| H | 0.00000000 | 0.00000000 | 4.00257355 |
| H | 0.00000000 | 3.97648410 | 1.44830201 |
| H | 0.00000000 | -3.97648410 | 1.44830201 |
| H | 0.00000000 | 2.56726559 | -3.47837232 |
| H | 0.00000000 | -2.56726559 | -3.47837232 |

## S1.99 Pyrrolopyrrole

CASRN: 250-87-3 (Pyrrolo[3,2-*b*]pyrrole)

Level of theory: CC3(FC)/cc-pVTZ

| | | | |
|---|---|---|---|
| C | 0.01987029 | 1.31191436 | 0.00000000 |
| C | -0.01987029 | -1.31191436 | 0.00000000 |
| C | -2.50055820 | 2.23026347 | 0.00000000 |
| C | 2.50055820 | -2.23026347 | 0.00000000 |
| C | -3.99867844 | 0.09474099 | 0.00000000 |
| C | 3.99867844 | -0.09474099 | 0.00000000 |
| N | 2.50780926 | 2.04699311 | 0.00000000 |
| N | -2.50780926 | -2.04699311 | 0.00000000 |
| H | -3.17172573 | 4.14262242 | 0.00000000 |

| | | | |
|---|---|---|---|
| H | 3.17172573 | -4.14262242 | 0.00000000 |
| H | -6.02037705 | -0.05658473 | 0.00000000 |
| H | 6.02037705 | 0.05658473 | 0.00000000 |
| H | 3.16071224 | 3.82066088 | 0.00000000 |
| H | -3.16071224 | -3.82066088 | 0.00000000 |

## S1.100 Quinoxaline

CASRN: 91-19-0

Level of theory: CC3(FC)/cc-pVTZ

| | | | |
|---|---|---|---|
| C | 0.00000000 | 1.33833541 | 0.04624026 |
| C | 0.00000000 | -1.33833541 | 0.04624026 |
| C | 0.00000000 | 2.65319151 | -2.27752466 |
| C | 0.00000000 | -2.65319151 | -2.27752466 |
| C | 0.00000000 | 1.33717941 | -4.51073479 |
| C | 0.00000000 | -1.33717941 | -4.51073479 |
| C | 0.00000000 | 1.33936683 | 4.32768896 |
| C | 0.00000000 | -1.33936683 | 4.32768896 |
| N | 0.00000000 | 2.68409862 | 2.24219152 |
| N | 0.00000000 | -2.68409862 | 2.24219152 |
| H | 0.00000000 | 4.68915946 | -2.22328575 |
| H | 0.00000000 | -4.68915946 | -2.22328575 |
| H | 0.00000000 | 2.33972888 | -6.28367426 |
| H | 0.00000000 | -2.33972888 | -6.28367426 |
| H | 0.00000000 | 2.35369837 | 6.10018213 |
| H | 0.00000000 | -2.35369837 | 6.10018213 |

## S1.101 $SiCl_2$

CASRN: 13569-32-9 (Dichlorosilylene)

Level of theory: CC3(Full)/*aug*-cc-pVTZ

| | | | |
|---|---|---|---|
| Si | 0.00000000 | 0.00000000 | -1.78528322 |
| Cl | 0.00000000 | 3.04414528 | 0.71619419 |
| Cl | 0.00000000 | -3.04414528 | 0.71619419 |

## S1.102 Silylidene

CASRN: 65632-07-7

Level of theory: CC3(Full)/*aug*-cc-pVTZ

| | | | |
|---|---|---|---|
| C | 0.00000000 | 0.00000000 | -2.09539928 |
| Si | 0.00000000 | 0.00000000 | 1.14992930 |
| H | 0.00000000 | 1.70929524 | -3.22894481 |
| H | 0.00000000 | -1.70929524 | -3.22894481 |

## S1.103 Streptocyanine-C1

CASRN:

Level of theory: CC3(Full)/*aug*-cc-pVTZ, Charge: +1

| | | | |
|---|---|---|---|
| C | 0.00000000 | 0.00000000 | 0.80488833 |
| N | 0.00000000 | 2.19423463 | -0.33580561 |
| N | 0.00000000 | -2.19423463 | -0.33580561 |
| H | 0.00000000 | 0.00000000 | 2.84436959 |
| H | 0.00000000 | 2.36978315 | -2.23371976 |
| H | 0.00000000 | -2.36978315 | -2.23371976 |
| H | 0.00000000 | 3.79412648 | 0.69399206 |
| H | 0.00000000 | -3.79412648 | 0.69399206 |

## S1.104 Streptocyanine-C3

CASRN:

Level of theory: CC3(Full)/*aug*-cc-pVTZ, Charge: +1

| | | | |
|---|---|---|---|
| C | 0.00000000 | 0.00000000 | 0.65419136 |
| C | 0.00000000 | 2.24294899 | -0.68901318 |
| C | 0.00000000 | -2.24294899 | -0.68901318 |
| N | 0.00000000 | 4.52279187 | 0.30876781 |
| N | 0.00000000 | -4.52279187 | 0.30876781 |
| H | 0.00000000 | 0.00000000 | 2.69658250 |
| H | 0.00000000 | 2.18484165 | -2.73430592 |
| H | 0.00000000 | -2.18484165 | -2.73430592 |
| H | 0.00000000 | 6.07453303 | -0.78935070 |
| H | 0.00000000 | -6.07453303 | -0.78935070 |
| H | 0.00000000 | 4.78699964 | 2.19452692 |
| H | 0.00000000 | -4.78699964 | 2.19452692 |

## S1.105 Streptocyanine-C5

CASRN:

Level of theory: CC3(Full)/cc-pVTZ, Charge: +1

| | | | |
|---|---|---|---|
| C | 0.00000000 | 0.00000000 | 0.46857445 |
| C | 0.00000000 | 2.33439812 | -0.72581892 |
| C | 0.00000000 | -2.33439812 | -0.72581892 |
| C | 0.00000000 | 4.51630408 | 0.70773577 |
| C | 0.00000000 | -4.51630408 | 0.70773577 |
| N | 0.00000000 | 6.84533147 | -0.19544059 |
| N | 0.00000000 | -6.84533147 | -0.19544059 |
| H | 0.00000000 | 0.00000000 | 2.51676448 |
| H | 0.00000000 | 2.44956750 | -2.76140399 |
| H | 0.00000000 | -2.44956750 | -2.76140399 |
| H | 0.00000000 | 4.36770843 | 2.74488884 |
| H | 0.00000000 | -4.36770843 | 2.74488884 |
| H | 0.00000000 | 8.34616080 | 0.96591148 |
| H | 0.00000000 | -8.34616080 | 0.96591148 |
| H | 0.00000000 | 7.18140877 | -2.06656349 |
| H | 0.00000000 | -7.18140877 | -2.06656349 |

## S1.106 Tetrathiafulvalene

CASRN: 31366-25-3

Level of theory: CC3(FC)/cc-pVTZ

| | | | |
|---|---|---|---|
| C | -1.27140171 | 0.00000000 | 0.00000000 |
| C | 1.27140171 | 0.00000000 | 0.00000000 |
| C | -5.98994256 | 1.26331812 | 0.00000000 |
| C | -5.98994256 | -1.26331812 | 0.00000000 |
| C | 5.98994256 | -1.26331812 | 0.00000000 |
| C | 5.98994256 | 1.26331812 | 0.00000000 |
| S | -3.07078317 | 2.82030107 | 0.00000000 |
| S | -3.07078317 | -2.82030107 | 0.00000000 |
| S | 3.07078317 | -2.82030107 | 0.00000000 |
| S | 3.07078317 | 2.82030107 | 0.00000000 |
| H | -7.66536437 | 2.41057807 | 0.00000000 |
| H | -7.66536437 | -2.41057807 | 0.00000000 |
| H | 7.66536437 | -2.41057807 | 0.00000000 |
| H | 7.66536437 | 2.41057807 | 0.00000000 |

## S1.107 Tetrazine

CASRN: 290-96-0 (*s*-Tetrazine)

Level of theory: CC3(Full)/*aug*-cc-pVTZ

| | | | |
|---|---|---|---|
| C | 0.00000000 | 0.00000000 | 2.38208164 |
| C | 0.00000000 | 0.00000000 | -2.38208164 |
| N | 2.25673244 | 0.00000000 | 1.24973261 |
| N | -2.25673244 | 0.00000000 | 1.24973261 |
| N | 2.25673244 | 0.00000000 | -1.24973261 |
| N | -2.25673244 | 0.00000000 | -1.24973261 |
| H | 0.00000000 | 0.00000000 | 4.41850901 |
| H | 0.00000000 | 0.00000000 | -4.41850901 |

## S1.108 Thienothiophene

CASRN: 251-41-2 (Thieno[3,2-*b*]thiophene)

Level of theory: CC3(FC)/cc-pVTZ

| | | | |
|---|---|---|---|
| C | 0.41618901 | 1.24091123 | 0.00000000 |
| C | -0.41618901 | -1.24091123 | 0.00000000 |
| C | -1.56128826 | 3.05660382 | 0.00000000 |
| C | 1.56128826 | -3.05660382 | 0.00000000 |
| C | -3.86882315 | 1.90421786 | 0.00000000 |
| C | 3.86882315 | -1.90421786 | 0.00000000 |
| S | 3.68518133 | 1.37661050 | 0.00000000 |
| S | -3.68518133 | -1.37661050 | 0.00000000 |
| H | -1.30761309 | 5.07161572 | 0.00000000 |
| H | 1.30761309 | -5.07161572 | 0.00000000 |
| H | -5.68944011 | 2.79705270 | 0.00000000 |
| H | 5.68944011 | -2.79705270 | 0.00000000 |

## S1.109 Thioacetone

CASRN: 4756-05-2 (2-Propanethione)

Level of theory: CC3(Full)/*aug*-cc-pVTZ

| | | | |
|---|---|---|---|
| C | 0.00000000 | 0.00000000 | 0.68476030 |
| C | 0.00000000 | 2.38541696 | 2.20685096 |
| C | 0.00000000 | -2.38541696 | 2.20685096 |
| S | 0.00000000 | 0.00000000 | -2.39920303 |

| | | | |
|---|---|---|---|
| H | 0.00000000 | 4.04609254 | 1.00090614 |
| H | 0.00000000 | -4.04609254 | 1.00090614 |
| H | 1.65894780 | 2.42602225 | 3.43712000 |
| H | -1.65894780 | 2.42602225 | 3.43712000 |
| H | 1.65894780 | -2.42602225 | 3.43712000 |
| H | -1.65894780 | -2.42602225 | 3.43712000 |

## S1.110 Thioacrolein

CASRN: 53439-64-8 (2-Propenethial)

Level of theory: CC3(Full)/*aug*-cc-pVTZ

| | | | |
|---|---|---|---|
| C | 4.27693176 | 0.00000000 | -0.88320133 |
| C | 1.76449030 | 0.00000000 | -1.23998444 |
| C | 0.00891877 | 0.00000000 | 0.85393278 |
| S | -3.06510749 | 0.00000000 | 0.58558716 |
| H | 5.57642075 | 0.00000000 | -2.45571463 |
| H | 5.06950243 | 0.00000000 | 1.00139499 |
| H | 0.96616458 | 0.00000000 | -3.11935314 |
| H | 0.87110201 | 0.00000000 | 2.71756937 |

## S1.111 Thioformaldehyde

CASRN: 865-36-1 (Methanethial)

Level of theory: CC3(Full)/*aug*-cc-pVTZ

Ground state

| | | | |
|---|---|---|---|
| C | 0.00000000 | 0.00000000 | -2.08677304 |
| S | 0.00000000 | 0.00000000 | 0.97251194 |
| H | 0.00000000 | 1.73657773 | -3.17013507 |
| H | 0.00000000 | -1.73657773 | -3.17013507 |

Excited state

| | | | |
|---|---|---|---|
| C | 0.00000000 | 0.00000000 | -2.20256705 |
| S | 0.00000000 | 0.00000000 | 1.02717172 |
| H | 0.00000000 | 1.76634191 | -3.21909384 |
| H | 0.00000000 | -1.76634191 | -3.21909384 |

## S1.112 Thioformaldehyde-S-oxide

CASRN: 40100-16-1 (Methanethial, S-oxide)

Level of theory: CC3(Full)/*aug*-cc-pVTZ

| | | | |
|---|---|---|---|
| C | -2.60499135 | 0.77983525 | 0.00000000 |
| O | 2.33211975 | 0.83760351 | 0.00000000 |
| S | 0.03093612 | -0.78961636 | 0.00000000 |
| H | -4.30439246 | -0.34582852 | 0.00000000 |
| H | -2.67226676 | 2.81674398 | 0.00000000 |

## S1.113 Thiophene

CASRN: 110-02-1

Level of theory: CC3(Full)/*aug*-cc-pVTZ

| | | | |
|---|---|---|---|
| C | 0.00000000 | 2.33342542 | -0.09858421 |
| C | 0.00000000 | -2.33342542 | -0.09858421 |
| C | 0.00000000 | 1.34371718 | -2.48297725 |
| C | 0.00000000 | -1.34371718 | -2.48297725 |
| S | 0.00000000 | 0.00000000 | 2.17250692 |
| H | 0.00000000 | 4.29028016 | 0.44577296 |
| H | 0.00000000 | -4.29028016 | 0.44577296 |
| H | 0.00000000 | 2.48760051 | -4.16768392 |
| H | 0.00000000 | -2.48760051 | -4.16768392 |

## S1.114 Thiopropynal

CASRN: 83797-21-1 (2-Propynethial)

Level of theory: CC3(Full)/*aug*-cc-pVTZ

| | | | |
|---|---|---|---|
| C | -0.00382924 | 0.00000000 | -1.25249909 |
| C | -2.27832423 | 0.00000000 | 0.15152736 |
| C | -4.26309583 | 0.00000000 | 1.29548793 |
| S | 2.81920288 | 0.00000000 | -0.00828974 |
| H | -0.23056990 | 0.00000000 | -3.28862183 |
| H | -5.97712967 | 0.00000000 | 2.33206931 |

## S1.115 Triazapentalene

CASRN: 431877-36-0 (1,3a,6a-Triazapentalene)

Level of theory: CC3(FC)/cc-pVTZ

| | | | |
|---|---|---|---|
| C | -2.50499953 | 2.11638523 | 0.00000000 |
| C | -3.96445816 | -0.07303868 | 0.00000000 |
| C | -2.35355924 | -2.15265577 | 0.00000000 |
| C | 3.83593935 | -0.03073106 | 0.00000000 |
| C | 2.43560744 | 2.16757403 | 0.00000000 |
| N | 0.04006152 | -1.21957559 | 0.00000000 |
| N | -0.04182459 | 1.35780418 | 0.00000000 |
| N | 2.39603035 | -2.14324663 | 0.00000000 |
| H | -3.00087038 | 4.07607227 | 0.00000000 |
| H | -5.98766760 | -0.14484657 | 0.00000000 |
| H | -2.68330099 | -4.14581320 | 0.00000000 |
| H | 5.85502782 | -0.19299220 | 0.00000000 |
| H | 2.92994089 | 4.12450552 | 0.00000000 |

## S1.116 Triazine

CASRN: 290-88-3 (*s*-Triazine)

Level of theory: CC3(Full)/*aug*-cc-pVTZ

| | | | |
|---|---|---|---|
| C | 0.00000000 | -2.11414732 | -1.22060353 |
| C | 0.00000000 | 0.00000000 | 2.44120705 |
| C | 0.00000000 | 2.11414732 | -1.22060353 |
| N | 0.00000000 | -2.24624733 | 1.29687150 |
| N | 0.00000000 | 2.24624733 | 1.29687150 |
| N | 0.00000000 | 0.00000000 | -2.59374300 |
| H | 0.00000000 | 3.88296710 | -2.24183210 |
| H | 0.00000000 | -3.88296710 | -2.24183210 |
| H | 0.00000000 | 0.00000000 | 4.48366420 |

## S1.117 Water

CASRN: 7732-18-5

Level of theory: CC3(Full)/*aug*-cc-pVTZ

| | | | |
|---|---|---|---|
| O | 0.00000000 | 0.00000000 | -0.13209669 |
| H | 0.00000000 | 1.43152878 | 0.97970006 |
| H | 0.00000000 | -1.43152878 | 0.97970006 |

# S2 RAD subset

## S2.1 $AlCH_2$

CASRN: 76392-50-2

Level of theory: RO-CCSD(T)(Full)/*aug*-cc-pVTZ

| | | | |
|---|---|---|---|
| Al | 0.00000000 | 0.00000000 | 0.00000000 |
| C | 0.00000000 | 0.00000000 | 3.71178683 |
| H | 1.67494363 | 0.00000000 | 4.90780205 |
| H | -1.67494363 | 0.00000000 | 4.90780205 |

## S2.2 Allyl

CASRN: 1981-80-2

Level of theory: U-CCSD(T)(Full)/*aug*-cc-pVTZ

| | | | |
|---|---|---|---|
| C | 0.00000000 | 0.00000000 | 0.84490222 |
| C | 0.00000000 | 2.30981224 | 0.37283352 |
| C | 0.00000000 | -2.30981224 | -0.37283352 |
| H | 0.00000000 | 0.00000000 | 2.88986557 |
| H | 0.00000000 | 4.06036949 | 0.67000051 |
| H | 0.00000000 | -4.06036949 | 0.67000051 |
| H | 0.00000000 | 2.41059890 | -2.41263791 |

## S2.3 BeF

CASRN: 13597-96-1

Level of theory: U-CCSD(T)(FC)/*aug*-cc-pVTZ [Only F's 1*s* frozen]

| | | | |
|---|---|---|---|
| Be | 0.00000000 | 0.00000000 | -1.77936990 |
| F | 0.00000000 | 0.00000000 | 0.79083149 |

## S2.4 BeH

CASRN: 13597-97-2

Level of theory: U-CCSD(T)(Full)/*aug*-cc-pVTZ

| | | | |
|---|---|---|---|
| Be | 0.00000000 | 0.00000000 | 0.25103976 |
| H | 0.00000000 | 0.00000000 | -2.24485003 |

## S2.5 $BH_2$

CASRN: 14452-64-3

Level of theory: U-CCSD(T)(Full)/*aug*-cc-pVTZ

| | | | |
|---|---|---|---|
| B | 0.00000000 | 0.00000000 | 0.14984923 |
| H | 0.00000000 | 2.01119016 | -0.81846345 |
| H | 0.00000000 | -2.01119016 | -0.81846345 |

## S2.6 $BO_2$

CASRN: 13840-88-5

Level of theory: U-CCSD(T)(Full)/*aug*-cc-pVTZ

| | | | |
|---|---|---|---|
| B | 0.00000000 | 0.00000000 | 0.00000000 |
| O | 0.00000000 | 0.00000000 | 2.39114228 |
| O | 0.00000000 | 0.00000000 | -2.39114228 |

## S2.7 CH

CASRN: 3315-37-5

Level of theory: U-CCSD(T)(Full)/*aug*-cc-pVTZ

| | | | |
|---|---|---|---|
| C | 0.00000000 | 0.00000000 | -0.16245872 |
| H | 0.00000000 | 0.00000000 | 1.93436816 |

## S2.8 $CH_2N$

CASRN: 15845-29-1

Level of theory: U-CCSD(T)(Full)/*aug*-cc-pVTZ

| | | | |
|---|---|---|---|
| N | 0.00000000 | 0.00000000 | 0.00000000 |
| C | 0.00000000 | 0.00000000 | 2.35340256 |
| H | 1.76354344 | 0.00000000 | 3.42267385 |
| H | -1.76354344 | 0.00000000 | 3.42267385 |

## S2.9 $CH_2O^+$

CASRN: 54288-05-0

Level of theory: U-CCSD(T)(Full)/*aug*-cc-pVTZ, Charge: +1

| | | | |
|---|---|---|---|
| O | 0.00000000 | 0.00000000 | 1.25868043 |
| C | 0.00000000 | 0.00000000 | -0.99972181 |
| H | 0.00000000 | 1.82487639 | -2.03556007 |
| H | 0.00000000 | -1.82487639 | -2.03556007 |

## S2.10 $CH_3$

CASRN: 2229-07-4

Level of theory: U-CCSD(T)(Full)/*aug*-cc-pVTZ

| | | | |
|---|---|---|---|
| C | 0.00000000 | 0.00000000 | 0.00000000 |
| H | 0.00000000 | 0.00000000 | 2.03379507 |
| H | 0.00000000 | 1.76131924 | -1.01689753 |
| H | 0.00000000 | -1.76131924 | -1.01689753 |

## S2.11 $ClO_2$

CASRN: 10049-04-4

Level of theory: U-CCSD(T)(Full)/*aug*-cc-pVTZ

| | | | |
|---|---|---|---|
| Cl | 0.00000000 | 0.00000000 | 0.70662178 |
| O | 0.00000000 | 2.40622607 | -0.77242528 |
| O | 0.00000000 | -2.40622607 | -0.77242528 |

## S2.12 CN

CASRN: 2074-87-5

Level of theory: U-CCSD(T)(Full)/*aug*-cc-pVTZ

| | | | |
|---|---|---|---|
| C | 0.00000000 | 0.00000000 | -1.18953886 |
| N | 0.00000000 | 0.00000000 | 1.01938091 |

## S2.13 CNO

CASRN: 1015843-63-6

Level of theory: U-CCSD(T)(Full)/*aug*-cc-pVTZ

| | | | |
|---|---|---|---|
| C | 0.00000000 | 0.00000000 | -2.50680714 |
| N | 0.00000000 | 0.00000000 | -0.22402176 |
| O | 0.00000000 | 0.00000000 | 2.07682752 |

## S2.14 $CO^+$

CASRN: 12144-04-6

Level of theory: U-CCSD(T)(Full)/*aug*-cc-pVTZ, Charge: +1

| | | | |
|---|---|---|---|
| C | 0.00000000 | 0.00000000 | -1.20324172 |
| O | 0.00000000 | 0.00000000 | 0.90271821 |

## S2.15 CON

CASRN: 162615-05-6

Level of theory: U-CCSDT(Full)/cc-pVTZ

| | | | |
|---|---|---|---|
| C | 0.00000000 | 0.00000000 | -2.44062558 |
| O | 0.00000000 | 0.00000000 | -0.20455596 |
| N | 0.00000000 | 0.00000000 | 2.32515818 |

## S2.16 Ethynyl

CASRN: 2122-48-7

Level of theory: U-CCSDT(Full)/*aug*-cc-pVTZ

| | | | |
|---|---|---|---|
| C | 0.00000000 | 0.00000000 | -1.01441459 |
| C | 0.00000000 | 0.00000000 | 1.26723128 |
| H | 0.00000000 | 0.00000000 | -3.01024506 |

## S2.17 $F_2BO$

CASRN: 38150-67-3

Level of theory: U-CCSDT(Full)/*aug*-cc-pVTZ

| | | | |
|---|---|---|---|
| O | 0.00000000 | 0.00000000 | 2.65260017 |
| B | 0.00000000 | 0.00000000 | 0.07681654 |
| F | 0.00000000 | 2.16433924 | -1.13888019 |
| F | 0.00000000 | -2.16433924 | -1.13888019 |

## S2.18 $F_2BS$

CASRN: 1643772-15-9

Level of theory: U-CCSDT(Full)/*aug*-cc-pVTZ

| | | | |
|---|---|---|---|
| S | 0.00000000 | 0.00000000 | 2.64960984 |
| B | 0.00000000 | 0.00000000 | -0.74406239 |
| F | 0.00000000 | 2.14169276 | -2.01390354 |
| F | 0.00000000 | -2.14169276 | -2.01390354 |

## S2.19 HBCl

CASRN: 158305-23-8

Level of theory: U-CCSDT(Full)/*aug*-cc-pVTZ

| | | | |
|---|---|---|---|
| H | -1.78942324 | 3.56349057 | 0.00000000 |
| B | 0.08133759 | 2.34034266 | 0.00000000 |
| Cl | 0.08133759 | -0.89795250 | 0.00000000 |

## S2.20 $H_2BO$

CASRN: 60448-21-7

Level of theory: U-CCSDT(Full)/*aug*-cc-pVTZ

| | | | |
|---|---|---|---|
| O | 0.00000000 | 0.00000000 | 1.17360276 |
| B | 0.00000000 | 0.00000000 | -1.27133435 |
| H | 0.00000000 | 1.98370787 | -2.36904602 |
| H | 0.00000000 | -1.98370787 | -2.36904602 |

## S2.21 HCO

CASRN: 2597-44-6

Level of theory: U-CCSDT(Full)/*aug*-cc-pVTZ

| | | | |
|---|---|---|---|
| H | 0.00000000 | -2.55038496 | 1.39798104 |
| C | 0.00000000 | -1.17300976 | -0.19046167 |
| O | 0.00000000 | 1.04073447 | 0.05480615 |

## S2.22 HOC

CASRN: 2597-44-6

Level of theory: U-CCSDT(Full)/*aug*-cc-pVTZ

| | | | |
|---|---|---|---|
| H | 0.00000000 | 1.82002973 | 1.50851586 |
| O | 0.00000000 | 0.96467865 | -0.12887834 |
| C | 0.00000000 | -1.43868535 | 0.04508983 |

## S2.23 $H_2PO$

CASRN: 97516-21-7

Level of theory: U-CCSD(T)(Full)/*aug*-cc-pVTZ

| | | | |
|---|---|---|---|
| P | 0.00000000 | 0.87766783 | -0.10010856 |
| O | 0.00000000 | -1.95912323 | 0.05701315 |
| H | 2.08101554 | 2.05955113 | 1.08591181 |
| H | -2.08101554 | 2.05955113 | 1.08591181 |

## S2.24 $H_2PS$

CASRN: 121022-96-6

Level of theory: U-CCSD(T)(Full)/*aug*-cc-pVTZ

| | | | |
|---|---|---|---|
| P | 0.00000000 | 1.81994516 | -0.10769248 |
| S | 0.00000000 | -1.93707861 | 0.02086846 |
| H | 2.03762554 | 2.75934101 | 1.32385757 |
| H | -2.03762554 | 2.75934101 | 1.32385757 |

## S2.25 $N_2^+$

CASRN: 13966-04-6

Level of theory: U-CCSD(T)(Full)/*aug*-cc-pVTZ, Charge: +1

| | | | |
|---|---|---|---|
| N | 0.00000000 | 0.00000000 | -1.05634935 |
| N | 0.00000000 | 0.00000000 | 1.05634935 |

## S2.26 NCO

CASRN: 22400-26-6

Level of theory: U-CCSD(T)(Full)/*aug*-cc-pVTZ

| | | | |
|---|---|---|---|
| N | 0.00000000 | 0.00000000 | -2.39343558 |
| C | 0.00000000 | 0.00000000 | -0.07238136 |
| O | 0.00000000 | 0.00000000 | 2.14968523 |

## S2.27 $NH_2$

CASRN: 13770-40-6

Level of theory: U-CCSD(T)(Full)/*aug*-cc-pVTZ

| | | | |
|---|---|---|---|
| N | 0.00000000 | 0.00000000 | 0.15111603 |
| H | 0.00000000 | 1.51574744 | -1.04982949 |
| H | 0.00000000 | -1.51574744 | -1.04982949 |

## S2.28 Nitromethyl

CASRN: 16787-85-2

Level of theory: U-CCSD(T)(Full)/*aug*-cc-pVTZ

| | | | |
|---|---|---|---|
| C | 0.00000000 | 0.00000000 | -2.58417104 |
| N | 0.00000000 | 0.00000000 | 0.08692471 |
| O | 0.00000000 | -2.06715629 | 1.15098225 |
| O | 0.00000000 | 2.06715629 | 1.15098225 |
| H | 0.00000000 | 1.81656349 | -3.48616378 |
| H | 0.00000000 | -1.81656349 | -3.48616378 |

## S2.29 NO

CASRN: 10102-43-9

Level of theory: U-CCSD(T)(Full)/*aug*-cc-pVTZ

| | | | |
|---|---|---|---|
| N | 0.00000000 | 0.00000000 | -1.15775086 |
| O | 0.00000000 | 0.00000000 | 1.01357658 |

## S2.30 $NO_2$

CASRN: 10102-44-0

Level of theory: U-CCSD(T)(Full)/*aug*-cc-pVTZ

| | | | |
|---|---|---|---|
| N | 0.00000000 | 0.00000000 | 0.60658130 |
| O | 0.00000000 | 2.08052421 | -0.26537991 |
| O | 0.00000000 | -2.08052421 | -0.26537991 |

## S2.31 OH

CASRN: 3352-57-6

Level of theory: U-CCSD(T)(Full)/*aug*-cc-pVTZ

| | | | |
|---|---|---|---|
| O | 0.00000000 | 0.00000000 | -0.10864763 |
| H | 0.00000000 | 0.00000000 | 1.72431679 |

## S2.32 $PH_2$

CASRN: 13765-43-0

Level of theory: U-CCSD(T)(Full)/*aug*-cc-pVTZ

| | | | |
|---|---|---|---|
| P | 0.00000000 | 0.00000000 | 0.11427641 |
| H | 0.00000000 | 1.91899987 | -1.75604411 |
| H | 0.00000000 | -1.91899987 | -1.75604411 |

## S2.33 Vinyl

CASRN: 2669-89-8

Level of theory: U-CCSD(T)(Full)/*aug*-cc-pVTZ

| | | | |
|---|---|---|---|
| C | 0.00000000 | 1.16769663 | -0.04303146 |
| C | 0.00000000 | -1.29945364 | 0.15810072 |
| H | 0.00000000 | 2.38429609 | 1.59801822 |
| H | 0.00000000 | 2.08759130 | -1.87998309 |
| H | 0.00000000 | -2.90307925 | -1.08814513 |

# S3 CHROM subset

## S3.1 Anthracene

CASRN: 120-12-7

Level of theory: CCSD(T)(FC)/cc-pVTZ

| | | | |
|---|---|---|---|
| C | 0.00000000 | 2.63580732 | 0.00000000 |
| C | 0.00000000 | -2.63580732 | 0.00000000 |
| C | -2.29791519 | 1.34956852 | 0.00000000 |
| C | 2.29791519 | 1.34956852 | 0.00000000 |
| C | -2.29791519 | -1.34956852 | 0.00000000 |
| C | 2.29791519 | -1.34956852 | 0.00000000 |
| C | -4.65745777 | 2.64726588 | 0.00000000 |
| C | 4.65745777 | 2.64726588 | 0.00000000 |
| C | -4.65745777 | -2.64726588 | 0.00000000 |
| C | 4.65745777 | -2.64726588 | 0.00000000 |
| C | -6.88218555 | 1.34593157 | 0.00000000 |
| C | 6.88218555 | 1.34593157 | 0.00000000 |
| C | -6.88218555 | -1.34593157 | 0.00000000 |
| C | 6.88218555 | -1.34593157 | 0.00000000 |
| H | 0.00000000 | 4.67946059 | 0.00000000 |
| H | 0.00000000 | -4.67946059 | 0.00000000 |
| H | -4.64776022 | 4.68790486 | 0.00000000 |
| H | 4.64776022 | 4.68790486 | 0.00000000 |
| H | -4.64776022 | -4.68790486 | 0.00000000 |
| H | 4.64776022 | -4.68790486 | 0.00000000 |
| H | -8.65488616 | 2.34873329 | 0.00000000 |
| H | 8.65488616 | 2.34873329 | 0.00000000 |
| H | -8.65488616 | -2.34873329 | 0.00000000 |
| H | 8.65488616 | -2.34873329 | 0.00000000 |

## S3.2 Anthraquinone

CASRN: 84-65-1 (9,10-Anthraquinone)

Level of theory: CCSD(T)(FC)/cc-pVTZ

| | | | |
|---|---|---|---|
| C | 0.00000000 | 2.77266798 | 0.00000000 |
| C | 0.00000000 | -2.77266798 | 0.00000000 |
| C | -2.39604276 | 1.31893403 | 0.00000000 |
| C | 2.39604276 | 1.31893403 | 0.00000000 |
| C | -2.39604276 | -1.31893403 | 0.00000000 |

| | | | |
|---|---|---|---|
| C | 2.39604276 | -1.31893403 | 0.00000000 |
| C | -4.67770721 | 2.63091924 | 0.00000000 |
| C | 4.67770721 | 2.63091924 | 0.00000000 |
| C | -4.67770721 | -2.63091924 | 0.00000000 |
| C | 4.67770721 | -2.63091924 | 0.00000000 |
| C | -6.94595480 | 1.31915183 | 0.00000000 |
| C | 6.94595480 | 1.31915183 | 0.00000000 |
| C | -6.94595480 | -1.31915183 | 0.00000000 |
| C | 6.94595480 | -1.31915183 | 0.00000000 |
| O | 0.00000000 | 5.07701524 | 0.00000000 |
| O | 0.00000000 | -5.07701524 | 0.00000000 |
| H | -4.62532501 | 4.66594073 | 0.00000000 |
| H | 4.62532501 | 4.66594073 | 0.00000000 |
| H | -4.62532501 | -4.66594073 | 0.00000000 |
| H | 4.62532501 | -4.66594073 | 0.00000000 |
| H | -8.70925236 | 2.33764025 | 0.00000000 |
| H | 8.70925236 | 2.33764025 | 0.00000000 |
| H | -8.70925236 | -2.33764025 | 0.00000000 |
| H | 8.70925236 | -2.33764025 | 0.00000000 |

## S3.3 Aza-BODIPY

CASRN: 934737-29-8

(Boron, difluoro[*N*-(2*H*-pyrrol-2-ylidene-$\kappa N$)-1*H*-pyrrol-2-aminato-$\kappa N^1$]-, (*T*-4))

Level of theory: CCSD(T)(FC)/cc-pVTZ

| | | | |
|---|---|---|---|
| B | 0.00000000 | 0.00000000 | 2.31704487 |
| C | 0.00000000 | 2.14450306 | -2.14127722 |
| C | 0.00000000 | -2.14450306 | -2.14127722 |
| C | 0.00000000 | 4.63460750 | -3.14651377 |
| C | 0.00000000 | -4.63460750 | -3.14651377 |
| C | 0.00000000 | 6.26996103 | -1.12023173 |
| C | 0.00000000 | -6.26996103 | -1.12023173 |
| C | 0.00000000 | 4.75475012 | 1.08608078 |
| C | 0.00000000 | -4.75475012 | 1.08608078 |
| N | 0.00000000 | 0.00000000 | -3.41527163 |
| N | 0.00000000 | 2.31056089 | 0.47890837 |
| N | 0.00000000 | -2.31056089 | 0.47890837 |
| F | -2.14709422 | 0.00000000 | 3.76825470 |
| F | 2.14709422 | 0.00000000 | 3.76825470 |
| H | 0.00000000 | 5.07027917 | -5.12686203 |
| H | 0.00000000 | -5.07027917 | -5.12686203 |

| | | | |
|---|---|---|---|
| H | 0.00000000 | 8.29623621 | -1.15574338 |
| H | 0.00000000 | -8.29623621 | -1.15574338 |
| H | 0.00000000 | 5.33784503 | 3.03195696 |
| H | 0.00000000 | -5.33784503 | 3.03195696 |

## S3.4 Azobenzene

CASRN: 103-33-3

Level of theory: CCSD(T)(FC)/cc-pVTZ

| | | | |
|---|---|---|---|
| N | 0.70983759 | 0.94706332 | 0.00000000 |
| N | -0.70983759 | -0.94706332 | 0.00000000 |
| C | 3.32897155 | 0.35325415 | 0.00000000 |
| C | -3.32897155 | -0.35325415 | 0.00000000 |
| C | 4.95331207 | 2.41934773 | 0.00000000 |
| C | -4.95331207 | -2.41934773 | 0.00000000 |
| C | 4.29774859 | -2.10116089 | 0.00000000 |
| C | -4.29774859 | 2.10116089 | 0.00000000 |
| C | 7.55507717 | 2.05070219 | 0.00000000 |
| C | -7.55507717 | -2.05070219 | 0.00000000 |
| C | 6.89206075 | -2.45941610 | 0.00000000 |
| C | -6.89206075 | 2.45941610 | 0.00000000 |
| C | 8.52712206 | -0.38973890 | 0.00000000 |
| C | -8.52712206 | 0.38973890 | 0.00000000 |
| H | 4.14639892 | 4.28913452 | 0.00000000 |
| H | -4.14639892 | -4.28913452 | 0.00000000 |
| H | 3.00966091 | -3.67317406 | 0.00000000 |
| H | -3.00966091 | 3.67317406 | 0.00000000 |
| H | 8.81009192 | 3.65424541 | 0.00000000 |
| H | -8.81009192 | -3.65424541 | 0.00000000 |
| H | 7.65006326 | -4.35029611 | 0.00000000 |
| H | -7.65006326 | 4.35029611 | 0.00000000 |
| H | 10.54199682 | -0.68600884 | 0.00000000 |
| H | -10.54199682 | 0.68600884 | 0.00000000 |

## S3.5 Bimane (*anti*)

CASRN: 77483-78-4 (1*H*,5*H*-Pyrazolo[1,2-*a*]pyrazole-1,5-dione)

Level of theory: CCSD(T)(FC)/cc-pVTZ

| | | | |
|---|---|---|---|
| N | 0.85541246 | -0.97258019 | -0.45355119 |

| | | | |
|---|---|---|---|
| N | -0.85541246 | 0.97258019 | -0.45355119 |
| C | 3.32393035 | -0.05259411 | 0.02808385 |
| C | -3.32393035 | 0.05259411 | 0.02808385 |
| C | 2.94286963 | 2.69259588 | 0.18980355 |
| C | -2.94286963 | -2.69259588 | 0.18980355 |
| C | 0.44568700 | 3.18647777 | -0.02731571 |
| C | -0.44568700 | -3.18647777 | -0.02731571 |
| O | 5.17687487 | -1.37077294 | 0.22137296 |
| O | -5.17687487 | 1.37077294 | 0.22137296 |
| H | 4.43821129 | 4.02646675 | 0.46706643 |
| H | -4.43821129 | -4.02646675 | 0.46706643 |
| H | -0.58057370 | 4.93386979 | 0.05227865 |
| H | 0.58057370 | -4.93386979 | 0.05227865 |

## S3.6 Bimane (*syn*)

CASRN: 79769-56-5 (1*H*,7*H*-Pyrazolo[1,2-*a*]pyrazole-1,7-dione)

Level of theory: CCSD(T)(FC)/cc-pVTZ

| | | | |
|---|---|---|---|
| N | -2.28025963 | -0.50360071 | 0.00000000 |
| N | 0.32822281 | -0.58012028 | 0.00000000 |
| C | 1.24260594 | -0.02312835 | 2.47750977 |
| C | 1.24260594 | -0.02312835 | -2.47750977 |
| C | -1.07959410 | 0.33452863 | 3.96056188 |
| C | -1.07959410 | 0.33452863 | -3.96056188 |
| C | -3.08345811 | 0.12284995 | 2.39997958 |
| C | -3.08345811 | 0.12284995 | -2.39997958 |
| O | 3.43458105 | 0.08666999 | 3.06946175 |
| O | 3.43458105 | 0.08666999 | -3.06946175 |
| H | -1.10355332 | 0.69492689 | 5.95117927 |
| H | -1.10355332 | 0.69492689 | -5.95117927 |
| H | -5.07134531 | 0.28781393 | 2.77255340 |
| H | -5.07134531 | 0.28781393 | -2.77255340 |

## S3.7 BODIPY

CASRN: 138026-71-8

(Boron, difluoro[2-[(2*H*-pyrrol-2-ylidene-$\kappa N$)methyl]-1*H*-pyrrolato-$\kappa N$]-, (*T*-4)-)

Level of theory: CCSD(T)(FC)/cc-pVTZ

| | | | |
|---|---|---|---|
| C | 0.00000000 | 0.00000000 | -3.45756235 |

| | | | |
|---|---|---|---|
| C | 0.00000000 | 2.28455780 | -2.18740413 |
| C | 0.00000000 | -2.28455780 | -2.18740413 |
| C | 0.00000000 | 4.79788592 | -3.09298460 |
| C | 0.00000000 | -4.79788592 | -3.09298460 |
| C | 0.00000000 | 6.36180283 | -0.99687598 |
| C | 0.00000000 | -6.36180283 | -0.99687598 |
| C | 0.00000000 | 4.76869637 | 1.13918303 |
| C | 0.00000000 | -4.76869637 | 1.13918303 |
| B | 0.00000000 | 0.00000000 | 2.22139632 |
| F | 2.14645956 | 0.00000000 | 3.68028136 |
| F | -2.14645956 | 0.00000000 | 3.68028136 |
| N | 0.00000000 | 2.34821228 | 0.42497916 |
| N | 0.00000000 | -2.34821228 | 0.42497916 |
| H | 0.00000000 | 5.33956943 | -5.04999407 |
| H | 0.00000000 | -5.33956943 | -5.04999407 |
| H | 0.00000000 | 8.38849882 | -0.96278552 |
| H | 0.00000000 | -8.38849882 | -0.96278552 |
| H | 0.00000000 | 5.26355675 | 3.10891537 |
| H | 0.00000000 | -5.26355675 | 3.10891537 |
| H | 0.00000000 | 0.00000000 | -5.49610864 |

## S3.8 Coumarin

CASRN: 91-64-5

Level of theory: CCSD(T)(FC)/cc-pVTZ

| | | | |
|---|---|---|---|
| C | -4.94880904 | -1.94740654 | 0.00000000 |
| C | -2.47093848 | -2.79532569 | 0.00000000 |
| C | -0.51937217 | -1.03691944 | 0.00000000 |
| C | -1.01215298 | 1.55096378 | 0.00000000 |
| C | -3.52597295 | 2.36676114 | 0.00000000 |
| C | -5.48705921 | 0.63898323 | 0.00000000 |
| C | 1.12079288 | 3.23364340 | 0.00000000 |
| C | 3.48627701 | 2.30671360 | 0.00000000 |
| C | 3.97501526 | -0.40562242 | 0.00000000 |
| O | 1.88373948 | -1.96225124 | 0.00000000 |
| O | 6.03004743 | -1.37035420 | 0.00000000 |
| H | -6.46892150 | -3.30170531 | 0.00000000 |
| H | -2.01507343 | -4.77869214 | 0.00000000 |
| H | -3.90920136 | 4.37002329 | 0.00000000 |
| H | -7.41766766 | 1.28158133 | 0.00000000 |
| H | 0.79237605 | 5.24728088 | 0.00000000 |
| H | 5.13342919 | 3.49535270 | 0.00000000 |

## S3.9 Cyclazine

CASRN: 519-61-9 (Cycl[3.3.3]azine)

Level of theory: CCSD(T)(FC)/cc-pVTZ

| | | | |
|---|---|---|---|
| C | 0.00000000 | -2.29619838 | 1.32571075 |
| C | 0.00000000 | -4.57380843 | -2.64068953 |
| C | 0.00000000 | 0.00000000 | -2.65142150 |
| C | 0.00000000 | 4.57380843 | -2.64068953 |
| C | 0.00000000 | 2.29619838 | 1.32571075 |
| C | 0.00000000 | 0.00000000 | 5.28137906 |
| C | 0.00000000 | -4.57334297 | -0.03501138 |
| C | 0.00000000 | 2.31699223 | -3.94312550 |
| C | 0.00000000 | 2.25635074 | 3.97813688 |
| C | 0.00000000 | -2.25635074 | 3.97813688 |
| C | 0.00000000 | -2.31699223 | -3.94312550 |
| C | 0.00000000 | 4.57334297 | -0.03501138 |
| N | 0.00000000 | 0.00000000 | 0.00000000 |
| H | 0.00000000 | 6.33829394 | -3.65941571 |
| H | 0.00000000 | 0.00000000 | 7.31883143 |
| H | 0.00000000 | -6.33829394 | -3.65941571 |
| H | 0.00000000 | -6.29930356 | 1.03947702 |
| H | 0.00000000 | 2.24943827 | -5.97509542 |
| H | 0.00000000 | 4.04986529 | 4.93561840 |
| H | 0.00000000 | -4.04986529 | 4.93561840 |
| H | 0.00000000 | -2.24943827 | -5.97509542 |
| H | 0.00000000 | 6.29930356 | 1.03947702 |

## S3.10 Diketopyrrolopyrrole

CASRN: 114482-12-1

Level of theory: CC3(FC)/cc-pVTZ

| | | | |
|---|---|---|---|
| C | -0.78095706 | 1.10654573 | 0.00000000 |
| C | 0.78095706 | -1.10654573 | 0.00000000 |
| C | 0.75770683 | 3.16221974 | 0.00000000 |
| C | -0.75770683 | -3.16221974 | 0.00000000 |
| C | -3.42805036 | 0.33490251 | 0.00000000 |
| C | 3.42805036 | -0.33490251 | 0.00000000 |
| N | -3.23354900 | -2.34444494 | 0.00000000 |
| N | 3.23354900 | 2.34444494 | 0.00000000 |
| O | -5.40649570 | 1.49154645 | 0.00000000 |
| O | 5.40649570 | -1.49154645 | 0.00000000 |

| | | | |
|---|---|---|---|
| H | -4.76571395 | -3.46112039 | 0.00000000 |
| H | 4.76571395 | 3.46112039 | 0.00000000 |
| H | 0.30840723 | 5.14301221 | 0.00000000 |
| H | -0.30840723 | -5.14301221 | 0.00000000 |

## S3.11 Heptazine

CASRN: 204-34-2 (1,3,4,6,7,9,9b-Heptaazaphenalene)

Level of theory: CCSD(T)(FC)/cc-pVTZ

| | | | |
|---|---|---|---|
| C | 0.00000000 | -2.28707566 | 1.32044375 |
| C | 0.00000000 | -4.25961422 | -2.45928942 |
| C | 0.00000000 | 0.00000000 | -2.64088750 |
| C | 0.00000000 | 4.25961422 | -2.45928942 |
| C | 0.00000000 | 2.28707566 | 1.32044375 |
| C | 0.00000000 | 0.00000000 | 4.91857884 |
| N | 0.00000000 | 0.00000000 | 0.00000000 |
| N | 0.00000000 | -4.45372767 | 0.04447145 |
| N | 0.00000000 | 2.18835043 | -3.87927703 |
| N | 0.00000000 | 2.26537724 | 3.83480558 |
| N | 0.00000000 | -2.26537724 | 3.83480558 |
| N | 0.00000000 | -2.18835043 | -3.87927703 |
| N | 0.00000000 | 4.45372767 | 0.04447145 |
| H | 0.00000000 | 6.02612802 | -3.47918663 |
| H | 0.00000000 | 0.00000000 | 6.95837327 |
| H | 0.00000000 | -6.02612802 | -3.47918663 |

## S3.12 Indacene

CASRN: 267-21-0 (*s*-Indacene)

Level of theory: CCSD(T)(FC)/cc-pVTZ

| | | | |
|---|---|---|---|
| C | -0.12187409 | 2.72754035 | 0.00000000 |
| C | 0.12187409 | -2.72754035 | 0.00000000 |
| C | -2.28967444 | 1.35454483 | 0.00000000 |
| C | 2.22799027 | 1.39213818 | 0.00000000 |
| C | 2.28967444 | -1.35454483 | 0.00000000 |
| C | -2.22799027 | -1.39213818 | 0.00000000 |
| C | -4.93933710 | 2.10101453 | 0.00000000 |
| C | 4.68186957 | 2.22844636 | 0.00000000 |
| C | 4.93933710 | -2.10101453 | 0.00000000 |

| | | | |
|---|---|---|---|
| C | -4.68186957 | -2.22844636 | 0.00000000 |
| C | 6.36303738 | 0.04329761 | 0.00000000 |
| C | -6.36303738 | -0.04329761 | 0.00000000 |
| H | -0.14271993 | 4.76943913 | 0.00000000 |
| H | 0.14271993 | -4.76943913 | 0.00000000 |
| H | -5.61765687 | 4.01700812 | 0.00000000 |
| H | 5.61765687 | -4.01700812 | 0.00000000 |
| H | 5.28839356 | 4.17123105 | 0.00000000 |
| H | -5.28839356 | -4.17123105 | 0.00000000 |
| H | 8.39157765 | 0.14300626 | 0.00000000 |
| H | -8.39157765 | -0.14300626 | 0.00000000 |

Level of theory: CCSD(T)(FC)/cc-pVTZ [$D_{2h}$ constrained]

| | | | |
|---|---|---|---|
| C | 0.00000000 | 2.70634052 | 0.00000000 |
| C | 0.00000000 | -2.70634052 | 0.00000000 |
| C | -2.25358383 | 1.35345832 | 0.00000000 |
| C | 2.25358383 | 1.35345832 | 0.00000000 |
| C | -2.25358383 | -1.35345832 | 0.00000000 |
| C | 2.25358383 | -1.35345832 | 0.00000000 |
| C | -4.81816884 | 2.15020878 | 0.00000000 |
| C | 4.81816884 | 2.15020878 | 0.00000000 |
| C | -4.81816884 | -2.15020878 | 0.00000000 |
| C | 4.81816884 | -2.15020878 | 0.00000000 |
| C | -6.36913809 | 0.00000000 | 0.00000000 |
| C | 6.36913809 | 0.00000000 | 0.00000000 |
| H | 0.00000000 | 4.74974165 | 0.00000000 |
| H | 0.00000000 | -4.74974165 | 0.00000000 |
| H | -5.45578565 | 4.08294742 | 0.00000000 |
| H | 5.45578565 | 4.08294742 | 0.00000000 |
| H | -5.45578565 | -4.08294742 | 0.00000000 |
| H | 5.45578565 | -4.08294742 | 0.00000000 |
| H | -8.39912836 | 0.00000000 | 0.00000000 |
| H | 8.39912836 | 0.00000000 | 0.00000000 |

## S3.13 Naphthalimide

CASRN: 81-83-4 (1,8-Naphthalimide)

Level of theory: CCSD(T)(FC)/cc-pVTZ

| | | | |
|---|---|---|---|
| C | 0.00000000 | 0.00000000 | 0.88414254 |
| C | 0.00000000 | 0.00000000 | 3.55510034 |
| C | 2.35632602 | 0.00000000 | -3.21426958 |

| | | | |
|---|---|---|---|
| C | -2.35632602 | 0.00000000 | -3.21426958 |
| C | 2.32275215 | 0.00000000 | -0.42671489 |
| C | -2.32275215 | 0.00000000 | -0.42671489 |
| C | 4.57007817 | 0.00000000 | 0.87369931 |
| C | -4.57007817 | 0.00000000 | 0.87369931 |
| C | 4.58083177 | 0.00000000 | 3.53384218 |
| C | -4.58083177 | 0.00000000 | 3.53384218 |
| C | 2.33984212 | 0.00000000 | 4.84532412 |
| C | -2.33984212 | 0.00000000 | 4.84532412 |
| N | 0.00000000 | 0.00000000 | -4.35793673 |
| O | 4.27090495 | 0.00000000 | -4.47823176 |
| O | -4.27090495 | 0.00000000 | -4.47823176 |
| H | 0.00000000 | 0.00000000 | -6.26502060 |
| H | 6.30814973 | 0.00000000 | -0.18744497 |
| H | -6.30814973 | 0.00000000 | -0.18744497 |
| H | 6.35338009 | 0.00000000 | 4.53440153 |
| H | -6.35338009 | 0.00000000 | 4.53440153 |
| H | 2.33715237 | 0.00000000 | 6.88533156 |
| H | -2.33715237 | 0.00000000 | 6.88533156 |

## S3.14 Naphthoquinone

CASRN: 130-15-4 (1,4-Naphthoquinone)

Level of theory: CCSD(T)(FC)/cc-pVTZ

| | | | |
|---|---|---|---|
| C | 0.00000000 | 1.31868219 | 5.07583353 |
| C | 0.00000000 | -1.31868219 | 5.07583353 |
| C | 0.00000000 | 2.63328396 | 2.80719633 |
| C | 0.00000000 | -2.63328396 | 2.80719633 |
| C | 0.00000000 | 1.31896773 | 0.52975242 |
| C | 0.00000000 | -1.31896773 | 0.52975242 |
| C | 0.00000000 | 2.74649968 | -1.88121997 |
| C | 0.00000000 | -2.74649968 | -1.88121997 |
| C | 0.00000000 | 1.26627836 | -4.24808471 |
| C | 0.00000000 | -1.26627836 | -4.24808471 |
| O | 0.00000000 | 5.05039066 | -1.94176133 |
| O | 0.00000000 | -5.05039066 | -1.94176133 |
| H | 0.00000000 | 2.33629038 | 6.83936996 |
| H | 0.00000000 | -2.33629038 | 6.83936996 |
| H | 0.00000000 | 4.66861735 | 2.75798976 |
| H | 0.00000000 | -4.66861735 | 2.75798976 |
| H | 0.00000000 | 2.35501749 | -5.96917497 |
| H | 0.00000000 | -2.35501749 | -5.96917497 |

## S3.15 Phenazine

CASRN: 92-82-0

Level of theory: CCSD(T)(FC)/cc-pVTZ

| | | | |
|---|---|---|---|
| N | 0.00000000 | 2.68425897 | 0.00000000 |
| N | 0.00000000 | -2.68425897 | 0.00000000 |
| C | -2.14725285 | 1.35123660 | 0.00000000 |
| C | 2.14725285 | 1.35123660 | 0.00000000 |
| C | -2.14725285 | -1.35123660 | 0.00000000 |
| C | 2.14725285 | -1.35123660 | 0.00000000 |
| C | -4.49864069 | 2.66174043 | 0.00000000 |
| C | 4.49864069 | 2.66174043 | 0.00000000 |
| C | -4.49864069 | -2.66174043 | 0.00000000 |
| C | 4.49864069 | -2.66174043 | 0.00000000 |
| C | -6.71414814 | 1.34756473 | 0.00000000 |
| C | 6.71414814 | 1.34756473 | 0.00000000 |
| C | -6.71414814 | -1.34756473 | 0.00000000 |
| C | 6.71414814 | -1.34756473 | 0.00000000 |
| H | -4.44549427 | 4.69771133 | 0.00000000 |
| H | 4.44549427 | 4.69771133 | 0.00000000 |
| H | -4.44549427 | -4.69771133 | 0.00000000 |
| H | 4.44549427 | -4.69771133 | 0.00000000 |
| H | -8.49075377 | 2.34322156 | 0.00000000 |
| H | 8.49075377 | 2.34322156 | 0.00000000 |
| H | -8.49075377 | -2.34322156 | 0.00000000 |
| H | 8.49075377 | -2.34322156 | 0.00000000 |

## S3.16 Phthalimide

CASRN: 85-41-6

Level of theory: CCSD(T)(FC)/cc-pVTZ

| | | | |
|---|---|---|---|
| C | 0.00000000 | 2.20210348 | 2.25054900 |
| C | 0.00000000 | -2.20210348 | 2.25054900 |
| C | 0.00000000 | 1.31050301 | -0.41254468 |
| C | 0.00000000 | -1.31050301 | -0.41254468 |
| C | 0.00000000 | 2.68001925 | -2.63336829 |
| C | 0.00000000 | -2.68001925 | -2.63336829 |
| C | 0.00000000 | 1.32018039 | -4.89183006 |
| C | 0.00000000 | -1.32018039 | -4.89183006 |
| N | 0.00000000 | 0.00000000 | 3.69708218 |
| O | 0.00000000 | 4.33361053 | 3.05657131 |

| | | | |
|---|---|---|---|
| O | 0.00000000 | -4.33361053 | 3.05657131 |
| H | 0.00000000 | 0.00000000 | 5.59565443 |
| H | 0.00000000 | 4.71538263 | -2.60774609 |
| H | 0.00000000 | -4.71538263 | -2.60774609 |
| H | 0.00000000 | 2.31561890 | -6.66791824 |
| H | 0.00000000 | -2.31561890 | -6.66791824 |

## S3.17 Tolan

CASRN: 501-65-5 (Diphenylacetylene)

Level of theory: CCSD(T)(FC)/cc-pVTZ

| | | | |
|---|---|---|---|
| C | -1.14632202 | 0.00000000 | 0.00000000 |
| C | 1.14632202 | 0.00000000 | 0.00000000 |
| C | -3.83802475 | 0.00000000 | 0.00000000 |
| C | 3.83802475 | 0.00000000 | 0.00000000 |
| C | -5.17616712 | -2.27953873 | 0.00000000 |
| C | -5.17616712 | 2.27953873 | 0.00000000 |
| C | 5.17616712 | 2.27953873 | 0.00000000 |
| C | 5.17616712 | -2.27953873 | 0.00000000 |
| C | -7.79943938 | -2.27513115 | 0.00000000 |
| C | -7.79943938 | 2.27513115 | 0.00000000 |
| C | 7.79943938 | 2.27513115 | 0.00000000 |
| C | 7.79943938 | -2.27513115 | 0.00000000 |
| C | -9.12002539 | 0.00000000 | 0.00000000 |
| C | 9.12002539 | 0.00000000 | 0.00000000 |
| H | -4.14659821 | -4.03713330 | 0.00000000 |
| H | -4.14659821 | 4.03713330 | 0.00000000 |
| H | 4.14659821 | 4.03713330 | 0.00000000 |
| H | 4.14659821 | -4.03713330 | 0.00000000 |
| H | -8.81141954 | -4.04290254 | 0.00000000 |
| H | -8.81141954 | 4.04290254 | 0.00000000 |
| H | 8.81141954 | 4.04290254 | 0.00000000 |
| H | 8.81141954 | -4.04290254 | 0.00000000 |
| H | -11.15613663 | 0.00000000 | 0.00000000 |
| H | 11.15613663 | 0.00000000 | 0.00000000 |

# S4 BIO subset

All five structures optimized within the $C_s$ point group.

## S4.1 Adenine

CASRN: 73-24-5

Level of theory: CCSD(T)(FC)/cc-pVTZ

| | | | |
|---|---|---|---|
| C | 4.34389426 | -1.33930557 | 0.00000000 |
| C | 0.36503408 | -0.97970268 | 0.00000000 |
| C | -2.26915710 | -1.24309632 | 0.00000000 |
| C | -2.53876831 | 3.08920859 | 0.00000000 |
| C | 1.28293141 | 1.47400078 | 0.00000000 |
| N | 3.85894777 | 1.21215063 | 0.00000000 |
| N | 2.30159967 | -2.73392473 | 0.00000000 |
| N | -3.39157056 | -3.52556500 | 0.00000000 |
| N | -3.70537008 | 0.83433013 | 0.00000000 |
| N | -0.07572621 | 3.60295597 | 0.00000000 |
| H | 6.24332770 | -2.05381037 | 0.00000000 |
| H | -5.28043911 | -3.62079788 | 0.00000000 |
| H | -2.33811893 | -5.09589359 | 0.00000000 |
| H | -3.78399739 | 4.70401819 | 0.00000000 |
| H | 5.12506600 | 2.62279018 | 0.00000000 |

## S4.2 Cytosine

CASRN: 71-30-7

Level of theory: CCSD(T)(FC)/cc-pVTZ

| | | | |
|---|---|---|---|
| C | 0.13153616 | -3.29434651 | 0.00000000 |
| C | -2.16958868 | -2.18889562 | 0.00000000 |
| C | -2.18164163 | 0.52447245 | 0.00000000 |
| C | 2.19656249 | 0.81672316 | 0.00000000 |
| N | 2.23905741 | -1.84899578 | 0.00000000 |
| N | -0.14418728 | 1.93350477 | 0.00000000 |
| N | -4.43045933 | 1.73167720 | 0.00000000 |
| O | 4.19248155 | 1.94651979 | 0.00000000 |
| H | 0.39918927 | -5.31187887 | 0.00000000 |
| H | -3.87818863 | -3.28205605 | 0.00000000 |
| H | 3.97074213 | -2.62813711 | 0.00000000 |

| | | | |
|---|---|---|---|
| H | -6.06514617 | 0.78792181 | 0.00000000 |
| H | -4.42374473 | 3.62537996 | 0.00000000 |

## S4.3 Guanine

CASRN: 73-40-5

Level of theory: CCSD(T)(FC)/cc-pVTZ

| | | | |
|---|---|---|---|
| C | 5.04300746 | 1.12824617 | 0.00000000 |
| C | 1.57302763 | -0.86835769 | 0.00000000 |
| C | -0.40267804 | -2.71708442 | 0.00000000 |
| C | -3.19825976 | 1.07461599 | 0.00000000 |
| C | 0.92432676 | 1.66261664 | 0.00000000 |
| N | 3.16411910 | 2.93199554 | 0.00000000 |
| N | 4.16277548 | -1.17626497 | 0.00000000 |
| N | -2.78865487 | -1.47177709 | 0.00000000 |
| N | -1.39530616 | 2.75841554 | 0.00000000 |
| N | -5.64049214 | 1.85006150 | 0.00000000 |
| O | -0.33087398 | -5.00601936 | 0.00000000 |
| H | 7.00588603 | 1.63926873 | 0.00000000 |
| H | 3.36597239 | 4.81669742 | 0.00000000 |
| H | -4.26765198 | -2.66994812 | 0.00000000 |
| H | -5.96845324 | 3.71127812 | 0.00000000 |
| H | -7.08863631 | 0.64037160 | 0.00000000 |

## S4.4 Thymine

CASRN: 65-71-4

Level of theory: CCSD(T)(FC)/cc-pVTZ

| | | | |
|---|---|---|---|
| C | -0.44648789 | -2.87628686 | 0.00000000 |
| C | -2.23106132 | -1.07024906 | 0.00000000 |
| C | -1.41814085 | 1.56526269 | 0.00000000 |
| C | 3.05578216 | 0.08300879 | 0.00000000 |
| C | -5.00077150 | -1.59149697 | 0.00000000 |
| N | 2.09834527 | -2.33675187 | 0.00000000 |
| N | 1.19471324 | 1.90812636 | 0.00000000 |
| O | -2.83684958 | 3.37116543 | 0.00000000 |
| O | 5.29613084 | 0.55170816 | 0.00000000 |
| H | -0.91267841 | -4.85754222 | 0.00000000 |
| H | 1.81222071 | 3.70986453 | 0.00000000 |

| | | | |
|---|---|---|---|
| H | 3.39365323 | -3.72203743 | 0.00000000 |
| H | -5.89402250 | -0.75236289 | 1.65133872 |
| H | -5.89402250 | -0.75236289 | -1.65133872 |
| H | -5.36530215 | -3.61421405 | 0.00000000 |

## S4.5 Uracil

CASRN: 66-22-8

Level of theory: CCSD(T)(FC)/cc-pVTZ

| | | | |
|---|---|---|---|
| C | 0.01392074 | -3.27902539 | 0.00000000 |
| C | -2.26233984 | -2.15421823 | 0.00000000 |
| C | -2.42555647 | 0.58974159 | 0.00000000 |
| C | 2.29689984 | 0.69433245 | 0.00000000 |
| N | 2.21975844 | -1.91565223 | 0.00000000 |
| N | -0.06699876 | 1.78681963 | 0.00000000 |
| O | -4.35746300 | 1.82310986 | 0.00000000 |
| O | 4.25135556 | 1.88203352 | 0.00000000 |
| H | 0.23773570 | -5.30086095 | 0.00000000 |
| H | -3.98274137 | -3.22402227 | 0.00000000 |
| H | -0.08859089 | 3.69140237 | 0.00000000 |
| H | 3.90983514 | -2.77633676 | 0.00000000 |

# S5 TM subset

## S5.1 CuCl

CASRN: 7758-89-6

Level of theory: CC3(FC)/*aug*-cc-pVTZ

```
Cu   0.00000000           0.00000000           0.00000000
Cl   0.00000000           0.00000000           3.92055750
```

## S5.2 CuF

CASRN: 13478-41-6

Level of theory: CC3(FC)/*aug*-cc-pVTZ

```
Cu   0.00000000           0.00000000           0.00000000
F    0.00000000           0.00000000           3.32142119
```

## S5.3 CuH

CASRN: 13517-00-5

Level of theory: CC3(FC)/*aug*-cc-pVTZ

```
Cu   0.00000000           0.00000000           0.00000000
H    0.00000000           0.00000000           2.79612230
```

## S5.4 ScF

CASRN: 14017-33-5

Level of theory: CC3(FC)/*aug*-cc-pVTZ

```
Sc   0.00000000           0.00000000           0.00000000
F    0.00000000           0.00000000           3.37830510
```

## S5.5 ScH

CASRN: 33486-02-1

Level of theory: CC3(FC)/*aug*-cc-pVTZ

| | | | |
|---|---|---|---|
| Sc | 0.00000000 | 0.00000000 | 0.00000000 |
| H | 0.00000000 | 0.00000000 | 3.39341243 |

## S5.6 ScO

CASRN: 12059-91-5

Level of theory: U-CCSD(T)(FC)/*aug*-cc-pVTZ

| | | | |
|---|---|---|---|
| Sc | 0.00000000 | 0.00000000 | -0.44577894 |
| O | 0.00000000 | 0.00000000 | 1.25292306 |

## S5.7 ScS

CASRN: 12294-10-9

Level of theory: U-CCSD(T)(FC)/*aug*-cc-pVTZ

| | | | |
|---|---|---|---|
| Sc | 0.00000000 | 0.00000000 | -0.90101143 |
| S | 0.00000000 | 0.00000000 | 1.26691157 |

## S5.8 TiN

CASRN: 25583-20-4

Level of theory: U-CCSD(T)(FC)/*aug*-cc-pVTZ

| | | | |
|---|---|---|---|
| Ti | 0.00000000 | 0.00000000 | -0.68309383 |
| N | 0.00000000 | 0.00000000 | 2.33898264 |

## S5.9 ZnH

CASRN: 13981-87-8

Level of theory: U-CCSD(T)(FC)/*aug*-cc-pVTZ

| | | | |
|---|---|---|---|
| Zn | 0.00000000 | 0.00000000 | -0.04701678 |
| H | 0.00000000 | 0.00000000 | 2.98240506 |

## S5.10 ZnO

CASRN: 1314-13-2

Level of theory: CC3(FC)/*aug*-cc-pVTZ

| | | | |
|---|---|---|---|
| Zn | 0.00000000 | 0.00000000 | 0.00000000 |
| O | 0.00000000 | 0.00000000 | 3.21175040 |

## S5.11 ZnS

CASRN: 1314-98-3

Level of theory: CC3(FC)/*aug*-cc-pVTZ

| | | | |
|---|---|---|---|
| Zn | 0.00000000 | 0.00000000 | 0.00000000 |
| S | 0.00000000 | 0.00000000 | 3.90705603 |
