# Supplementary material for: The QUEST Database of Highly-Accurate Excitation Energies
Source: arXiv:2506.11590 ancillary file (2025-07-28)
Supplement: Supplementary file 2 [file QUEST-SI-Other.pdf]

# SI for
# The QUEST Database of Highly-Accurate Excitation Energies: Extra Data and Analysis

Pierre-François Loos,*,† Martial Boggio-Pasqua,† Aymeric Blondel,‡ Filippo Lipparini,¶ and Denis Jacquemin*,‡,§

†*Laboratoire de Chimie et Physique Quantiques, Université de Toulouse, CNRS, F-31062 Toulouse, France*

‡*Nantes Université, CNRS, CEISAM UMR 6230, F-44000 Nantes, France*

¶*Dipartimento di Chimica e Chimica Industriale, University of Pisa, Via Moruzzi 3, 56124 Pisa, Italy*

§*Institut Universitaire de France (IUF), F-75005 Paris, France*

E-mail: loos@irsamc.ups-tlse.fr; Denis.Jacquemin@univ-nantes.fr

# S1 Detailed content per subset

## S1.1 Closed-shell organic compounds

Table S1: Number of TBEs in the various subsets of closed-shell molecules detailed by category. Mixed indicates ESs with strong valence/Rydberg mixing.

| | MAIN | | | | | |
|---|---|---|---|---|---|---|
| | | Singlet | | | Triplet | |
| Size (non-H atoms) | Valence | Rydberg | Mixed | Valence | Rydberg | Mixed |
| Tiny (1–2) | 45 | 28 | 2 | 35 | 19 | 0 |
| Small (3–5) | 112 | 76 | 2 | 100 | 28 | 0 |
| Medium (6–9) | 145 | 75 | 3 | 105 | 10 | 0 |
| Large (10–16) | 74 | 19 | 1 | 43 | 4 | 1 |
| | CHROM | | | | | |
| | | Singlet | | | Triplet | |
| Size (non-H atoms) | Valence | Rydberg | Mixed | Valence | Rydberg | Mixed |
| Tiny (1–2) | 0 | 0 | 0 | 0 | 0 | 0 |
| Small (3–5) | 0 | 0 | 0 | 0 | 0 | 0 |
| Medium (6–9) | 0 | 0 | 0 | 0 | 0 | 0 |
| Large (10–16) | 79 | 7 | 0 | 70 | 2 | 0 |
| | BIO | | | | | |
| | | Singlet | | | Triplet | |
| Size (non-H atoms) | Valence | Rydberg | Mixed | Valence | Rydberg | Mixed |
| Tiny (1–2) | 0 | 0 | 0 | 0 | 0 | 0 |
| Small (3–5) | 0 | 0 | 0 | 0 | 0 | 0 |
| Medium (6–9) | 16 | 5 | 0 | 9 | 3 | 0 |
| Large (10–16) | 9 | 5 | 0 | 6 | 3 | 0 |
| | TOTAL | | | | | |
| | | Singlet | | | Triplet | |
| Size (non-H atoms) | Valence | Rydberg | Mixed | Valence | Rydberg | Mixed |
| Tiny (1–2) | 45 | 28 | 2 | 35 | 19 | 0 |
| Small (3–5) | 112 | 76 | 2 | 100 | 28 | 0 |
| Medium (6–9) | 161 | 80 | 3 | 114 | 13 | 0 |
| Large (10–16) | 157 | 31 | 1 | 119 | 9 | 1 |

Table S2: Number of TBEs in the RAD subset detailed by category. Mixed indicates ESs with strong valence/Rydberg mixing.

| | RAD | | | | | |
|---|---|---|---|---|---|---|
| | | Doublet | | | Quartet | |
| Size (non-H atoms) | Valence | Rydberg | Mixed | Valence | Rydberg | Mixed |
| Tiny (1–2) | 76 | 62 | 18 | 31 | 7 | 7 |
| Small (3–5) | 44 | 10 | 7 | 15 | 3 | 1 |

# S2 Extra basis set analyses

## S2.1 Closed-shell compounds

Table S3: Average (MSE and MAE in eV) errors obtained with 6-31+G(d) as compared to AVTZ at the CC3 level for all non-genuine-double ESs contained in the MAIN, CHROM, and BIO subsets.

| States | MSE | MAE |
|---|---|---|
| All | 0.113 | 0.118 |
| | | |
| Valence | 0.101 | 0.104 |
| $n\pi^\star$ | 0.100 | 0.101 |
| $\pi\pi^\star$ | 0.104 | 0.107 |
| Rydberg | 0.144 | 0.158 |
| | | |
| Singlet | 0.137 | 0.141 |
| Triplet | 0.068 | 0.077 |
| | | |
| Tiny | 0.164 | 0.173 |
| Small | 0.092 | 0.103 |
| Medium | 0.123 | 0.126 |
| Large | 0.106 | 0.108 |

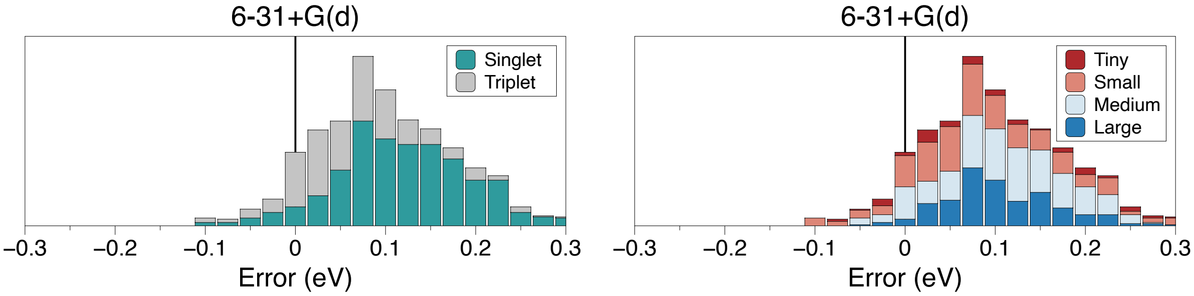


Figure S1: Distribution of the errors as compared to the AVTZ VTEs when using 6-31+G(d). All calculations at the CC3 level considering all (non-gd) ESs of the MAIN, CHROM and BIO subsets.

Table S4: Average (MSE and MAE in eV) errors obtained with AVDZ as compared to AVTZ at the CC3 level for all non-genuine-double ESs contained in the MAIN, CHROM and BIO subsets.

| States | MSE | MAE |
|---|---|---|
| All | 0.007 | 0.048 |
| | | |
| Valence | 0.032 | 0.034 |
| $n\pi^\star$ | 0.029 | 0.031 |
| $\pi\pi^\star$ | 0.034 | 0.035 |
| Rydberg | -0.063 | 0.086 |
| | | |
| Singlet | 0.009 | 0.055 |
| Triplet | 0.004 | 0.036 |
| | | |
| Tiny | 0.022 | 0.078 |
| Small | -0.002 | 0.050 |
| Medium | 0.005 | 0.046 |
| Large | 0.013 | 0.033 |

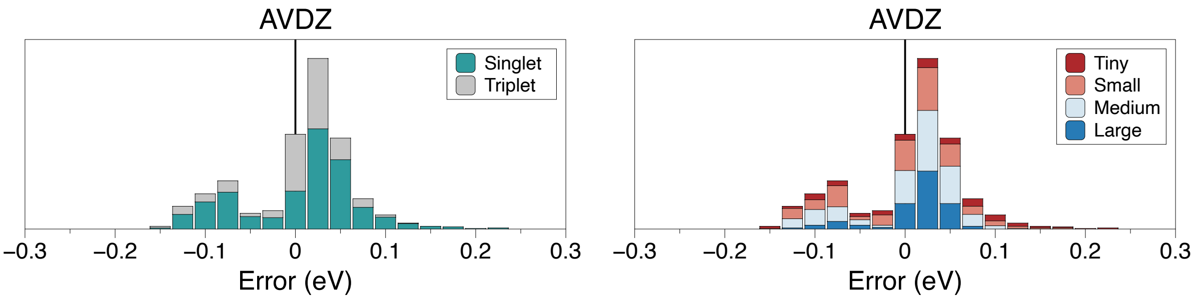


Figure S2: Distribution of the errors as compared to the AVTZ VTEs when using AVDZ. All calculations at the CC3 level considering all (non-gd) ESs of the MAIN, CHROM and BIO subsets

Table S5: Average (MSE and MAE in eV) differences obtained with AVQZ as compared to AVTZ at the CC3 level for all non-genuine-double ESs contained in the MAIN subset.

| States | MSE | MAE |
|---|---|---|
| All | 0.007 | 0.018 |
| | | |
| Valence | 0.002 | 0.009 |
| $n\pi^\star$ | 0.003 | 0.010 |
| $\pi\pi^\star$ | 0.001 | 0.008 |
| Rydberg | 0.017 | 0.037 |
| | | |
| Singlet | 0.003 | 0.020 |
| Triplet | 0.012 | 0.014 |
| | | |
| Tiny | 0.001 | 0.026 |
| Small | 0.009 | 0.017 |
| Medium | 0.006 | 0.012 |
| Large | – | – |

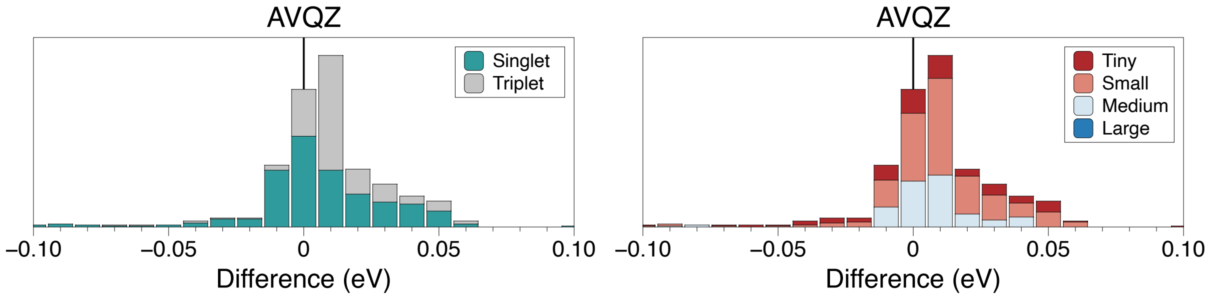


Figure S3: Distribution of the differences as compared to the AVTZ VTEs when using AVQZ. All calculations at the CC3 level considering all (non-gd) ESs of the MAIN subset.

## S2.2 Open-shell compounds

Table S6: Average (MSE and MAE in eV) errors obtained with 6-31+G(d) as compared to AVTZ at the CC3 level for all non-genuine-double ESs contained in the RAD subset.

| States | MSE | MAE |
|---|---|---|
| All | 0.089 | 0.123 |
| | | |
| Valence | 0.060 | 0.087 |
| Rydberg | 0.128 | 0.180 |
| Mixed | 0.138 | 0.171 |
| | | |
| Doublet | 0.112 | 0.133 |
| Quartet | 0.019 | 0.093 |
| | | |
| Tiny | 0.105 | 0.137 |
| Small | 0.049 | 0.091 |

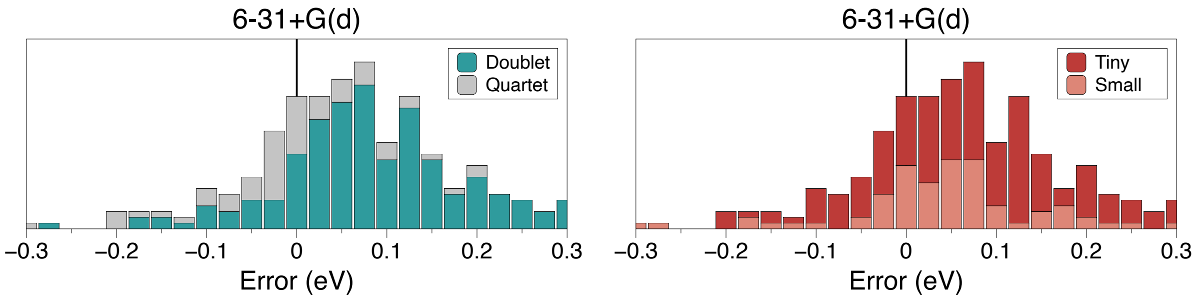


Figure S4: Distribution of the errors as compared to the AVTZ VTEs when using 6-31+G(d). All calculations at the CC3 level considering all (non-gd) ESs of the RAD subset.

Table S7: Average (MSE and MAE in eV) errors obtained with AVDZ as compared to AVTZ at the CC3 level for all non-genuine-double ESs contained in the RAD subset.

| States | MSE | MAE |
|---|---|---|
| All | 0.016 | 0.060 |
| | | |
| Valence | 0.025 | 0.042 |
| Rydberg | -0.008 | 0.093 |
| Mixed | 0.033 | 0.062 |
| | | |
| Doublet | 0.029 | 0.063 |
| Quartet | -0.025 | 0.050 |
| | | |
| Tiny | 0.019 | 0.066 |
| Small | 0.009 | 0.046 |

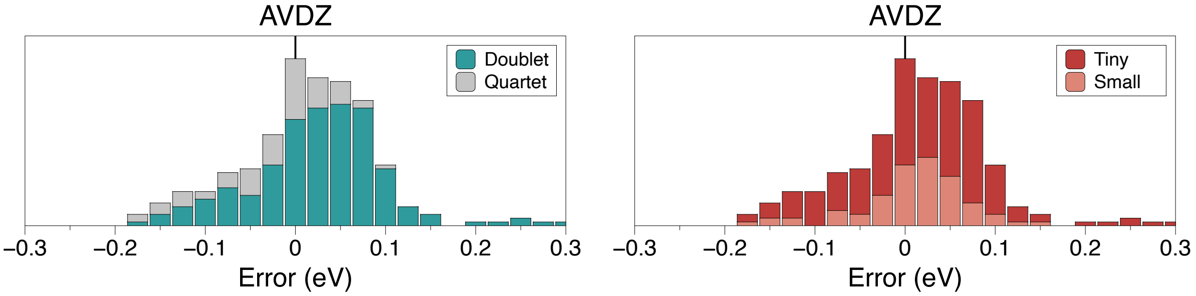


Figure S5: Distribution of the errors as compared to the AVTZ VTEs when using AVDZ. All calculations at the CC3 level considering all (non-gd) ESs of the RAD subset.

Table S8: Average (MSE and MAE in eV) differences obtained with AVQZ as compared to AVTZ at the CC3 level for all non-genuine-double ESs contained in the RAD subset.

| States | MSE | MAE |
|---|---|---|
| All | -0.004 | 0.021 |
| | | |
| Valence | 0.001 | 0.011 |
| Rydberg | -0.014 | 0.038 |
| Mixed | -0.002 | 0.019 |
| | | |
| Doublet | -0.010 | 0.022 |
| Quartet | 0.017 | 0.018 |
| | | |
| Tiny | -0.005 | 0.022 |
| Small | 0.005 | 0.012 |

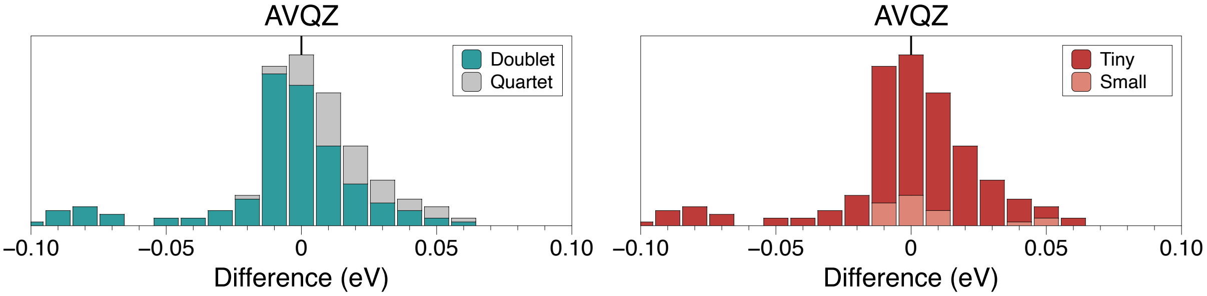


Figure S6: Distribution of the differences as compared to the AVQZ VTEs when using 6-31+G(d). All calculations at the CC3 level considering all (non-gd) ESs of the RAD subset.

# S3 Additional benchmark graphs

## S3.1 Closed-shell compounds

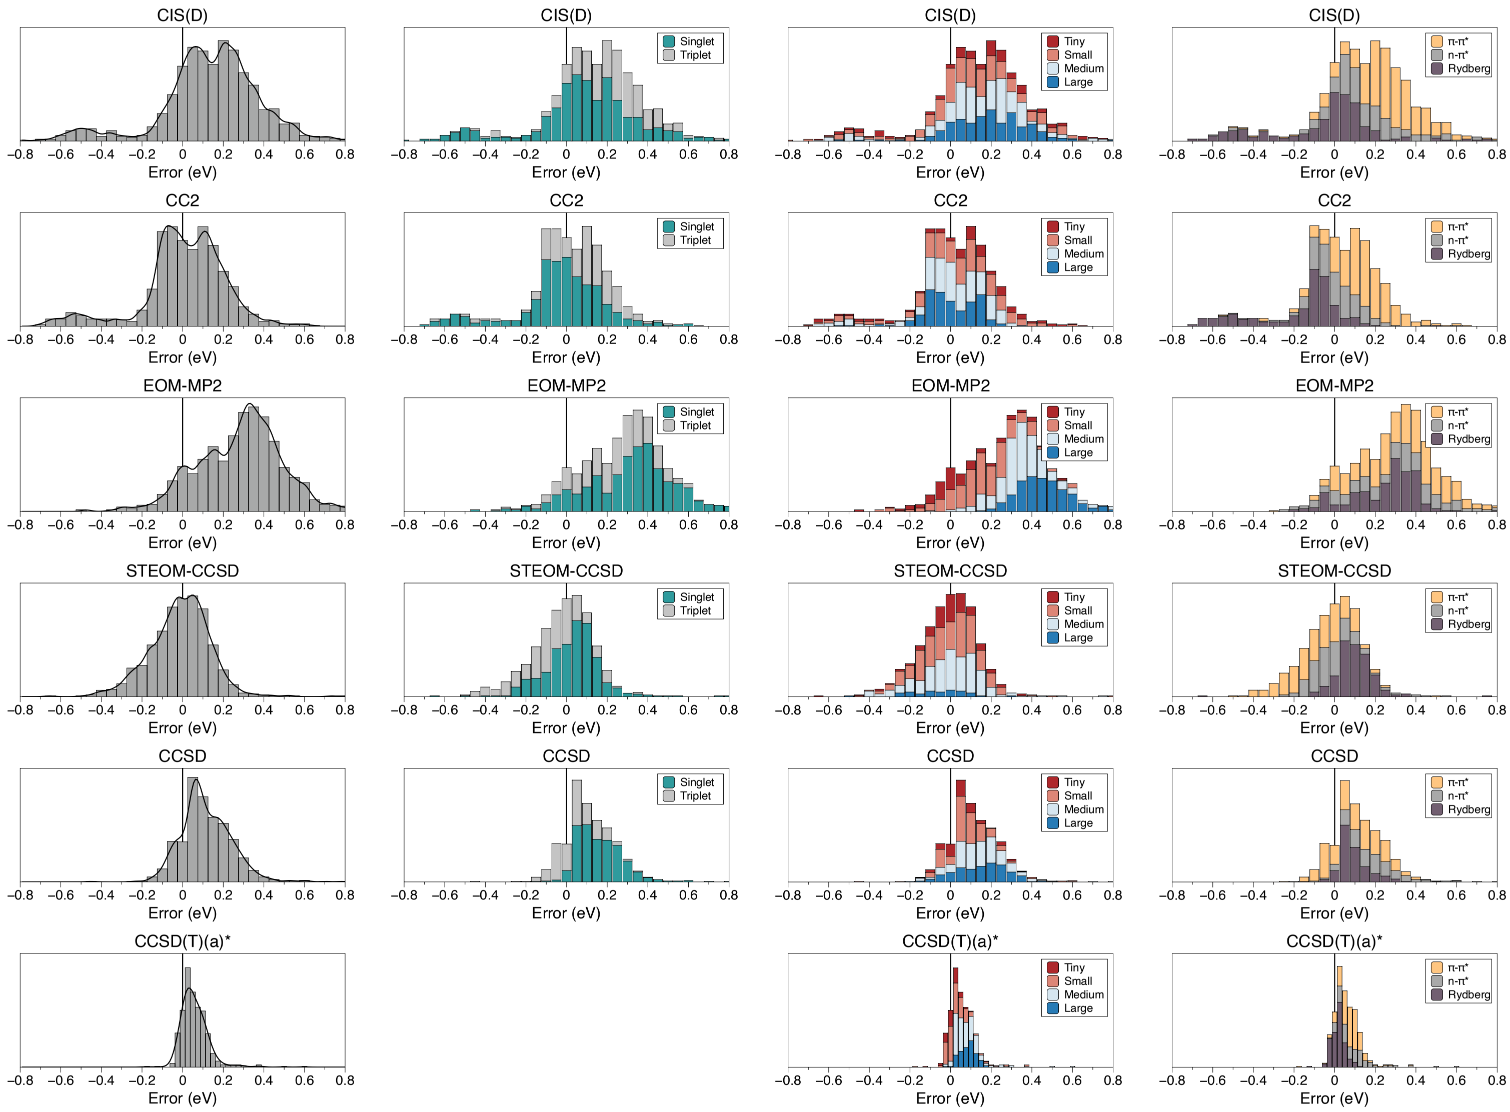


Figure S7: Distribution of the errors on VTEs for selected methods considering all safe and non-GD data in the of MAIN, CHROM and BIO subsets. From left to right: all transitions, impact of the spin symmetry, influence of molecular size, and effect of ES nature.

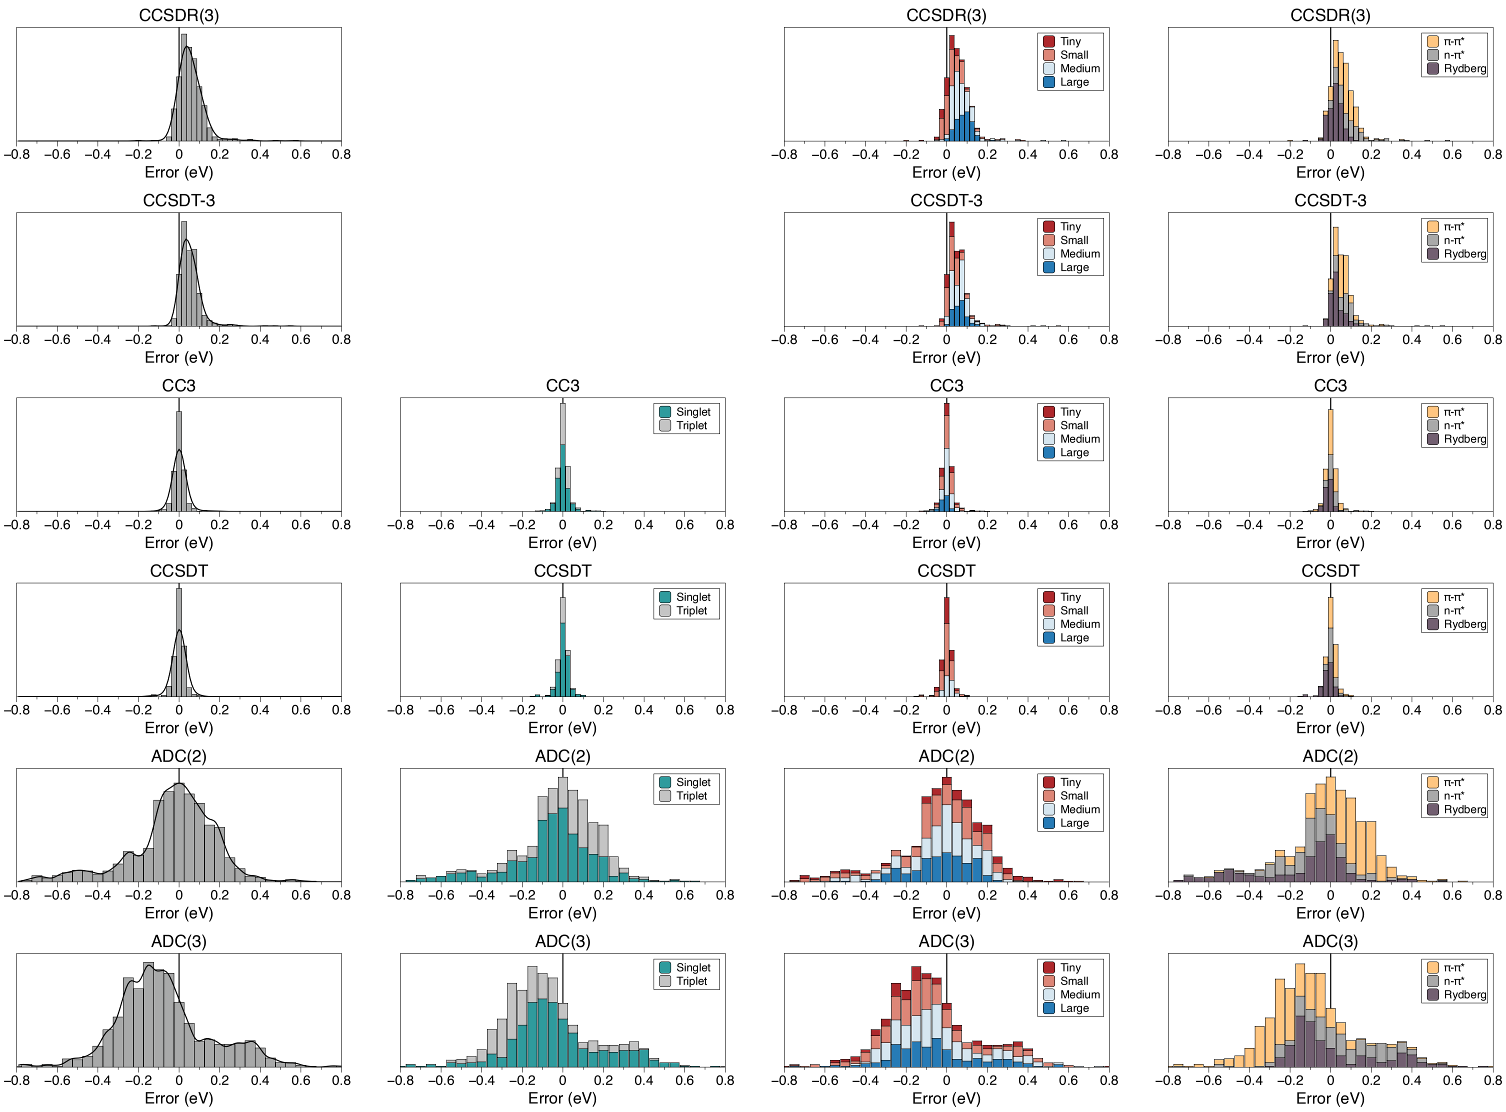


Figure S8: Distribution of the errors on VTEs for selected methods considering all safe and non-GD data in the of MAIN, CHROM and BIO subsets. From left to right: all transitions, impact of the spin symmetry, influence of molecular size, and effect of ES nature.

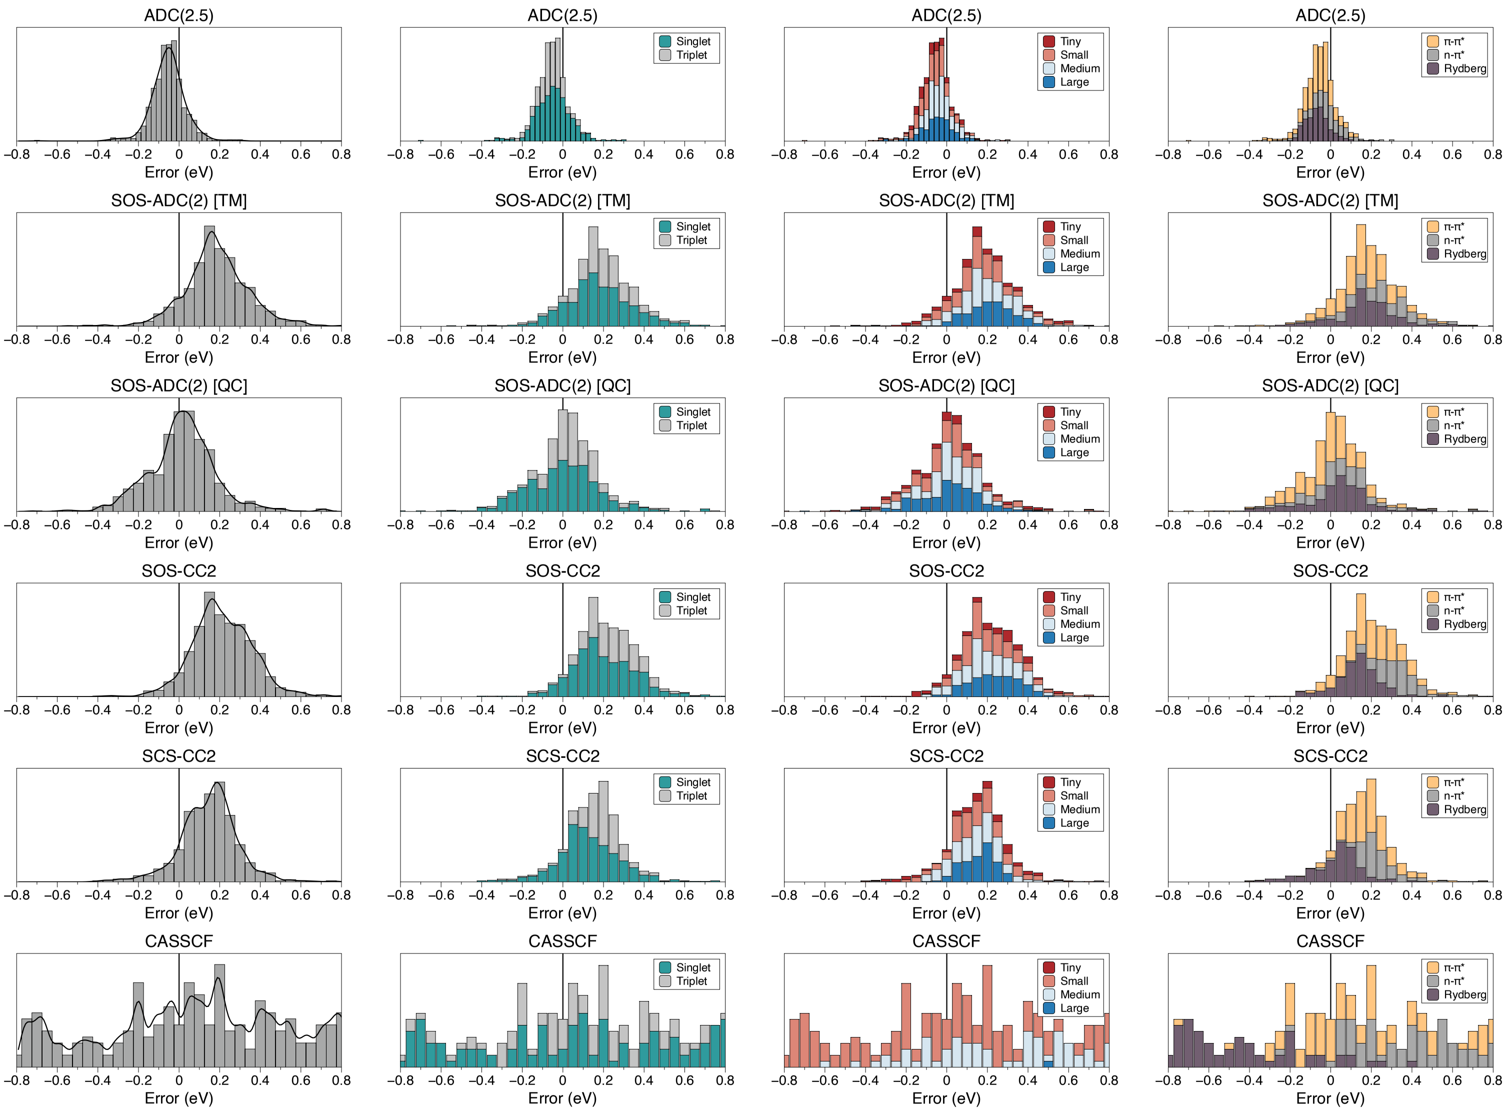


Figure S9: Distribution of the errors on VTEs for selected methods considering all safe and non-GD data in the of MAIN, CHROM and BIO subsets. From left to right: all transitions, impact of the spin symmetry, influence of molecular size, and effect of ES nature.

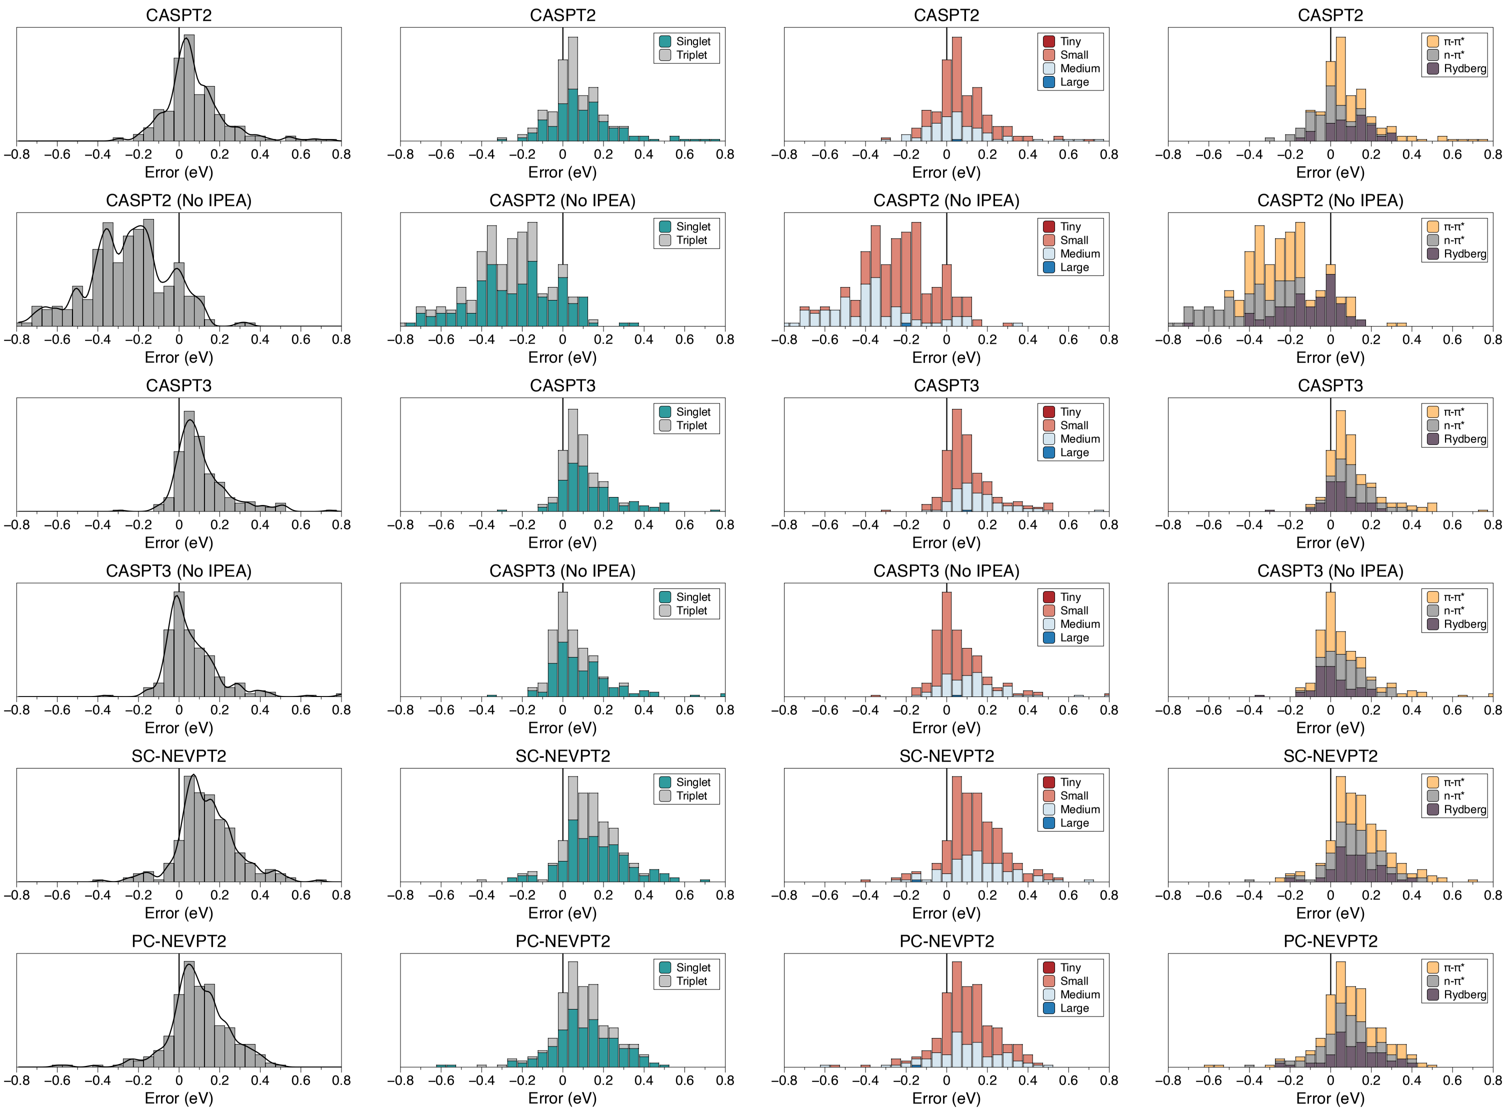


Figure S10: Distribution of the errors on VTEs for selected methods considering all safe and non-GD data in the of MAIN, CHROM and BIO subsets. From left to right: all transitions, impact of the spin symmetry, influence of molecular size, and effect of ES nature.

## S3.2 Open-shell compounds

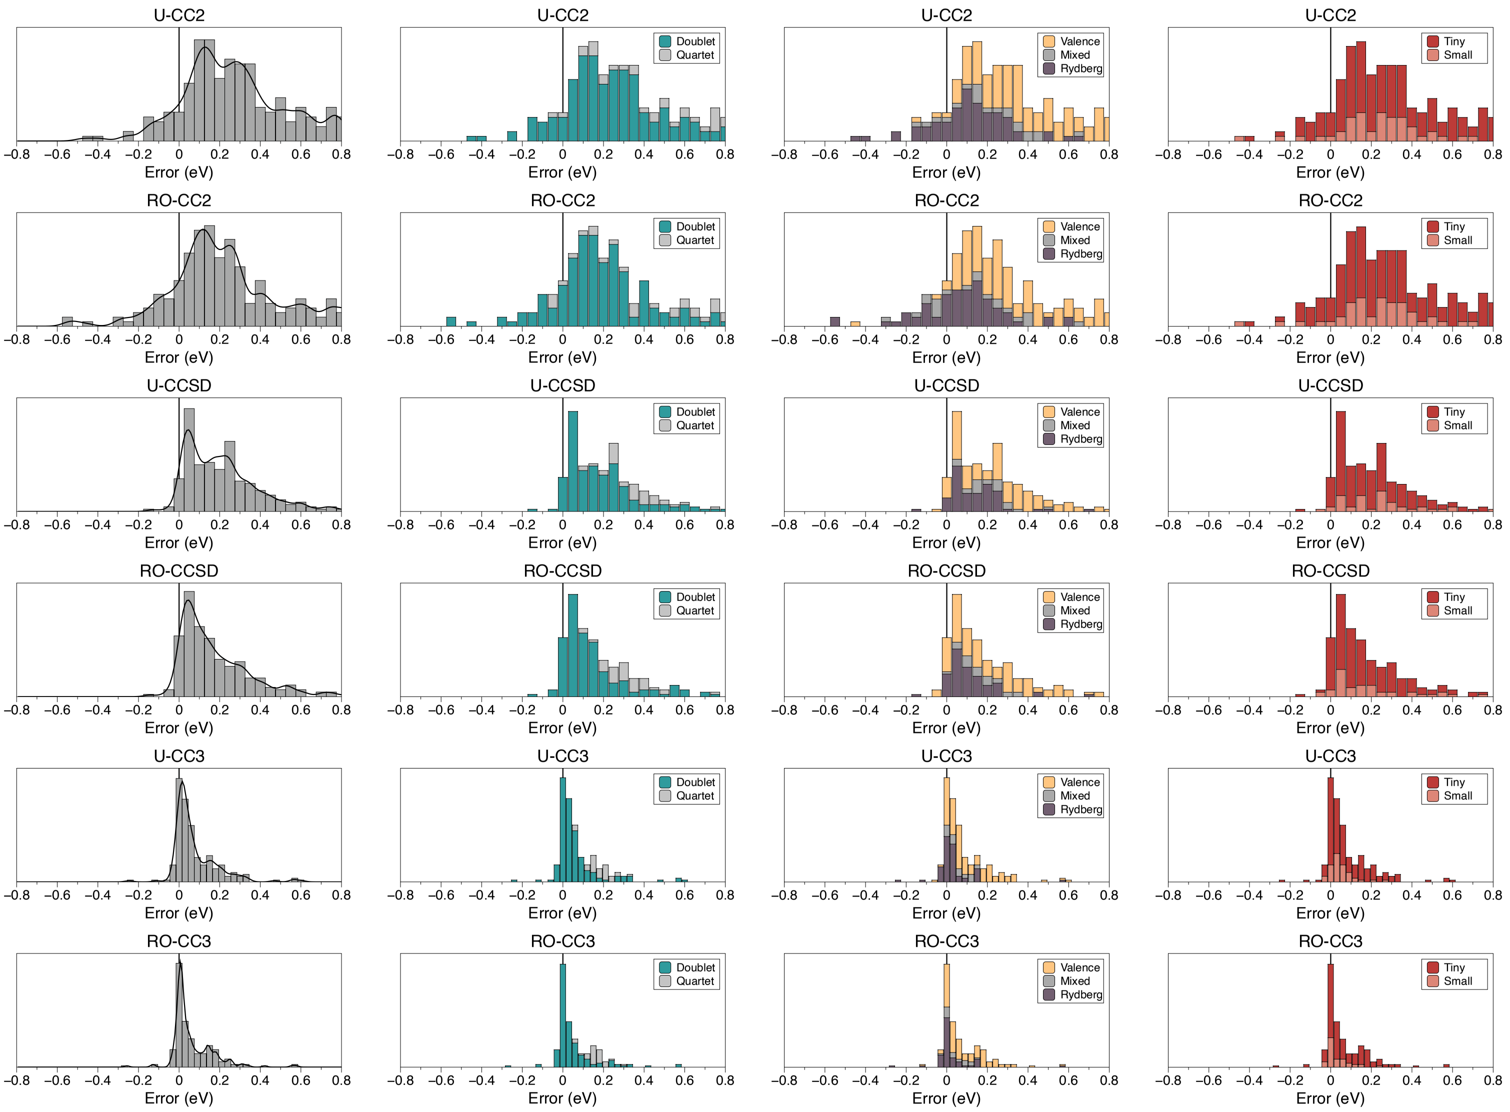

Figure S11: Distribution of the errors on VTEs for selected methods considering all safe and non-GD data in the of RAD subset. From left to right: all transitions, impact of the spin symmetry, influence of molecular size, and effect of ES nature.

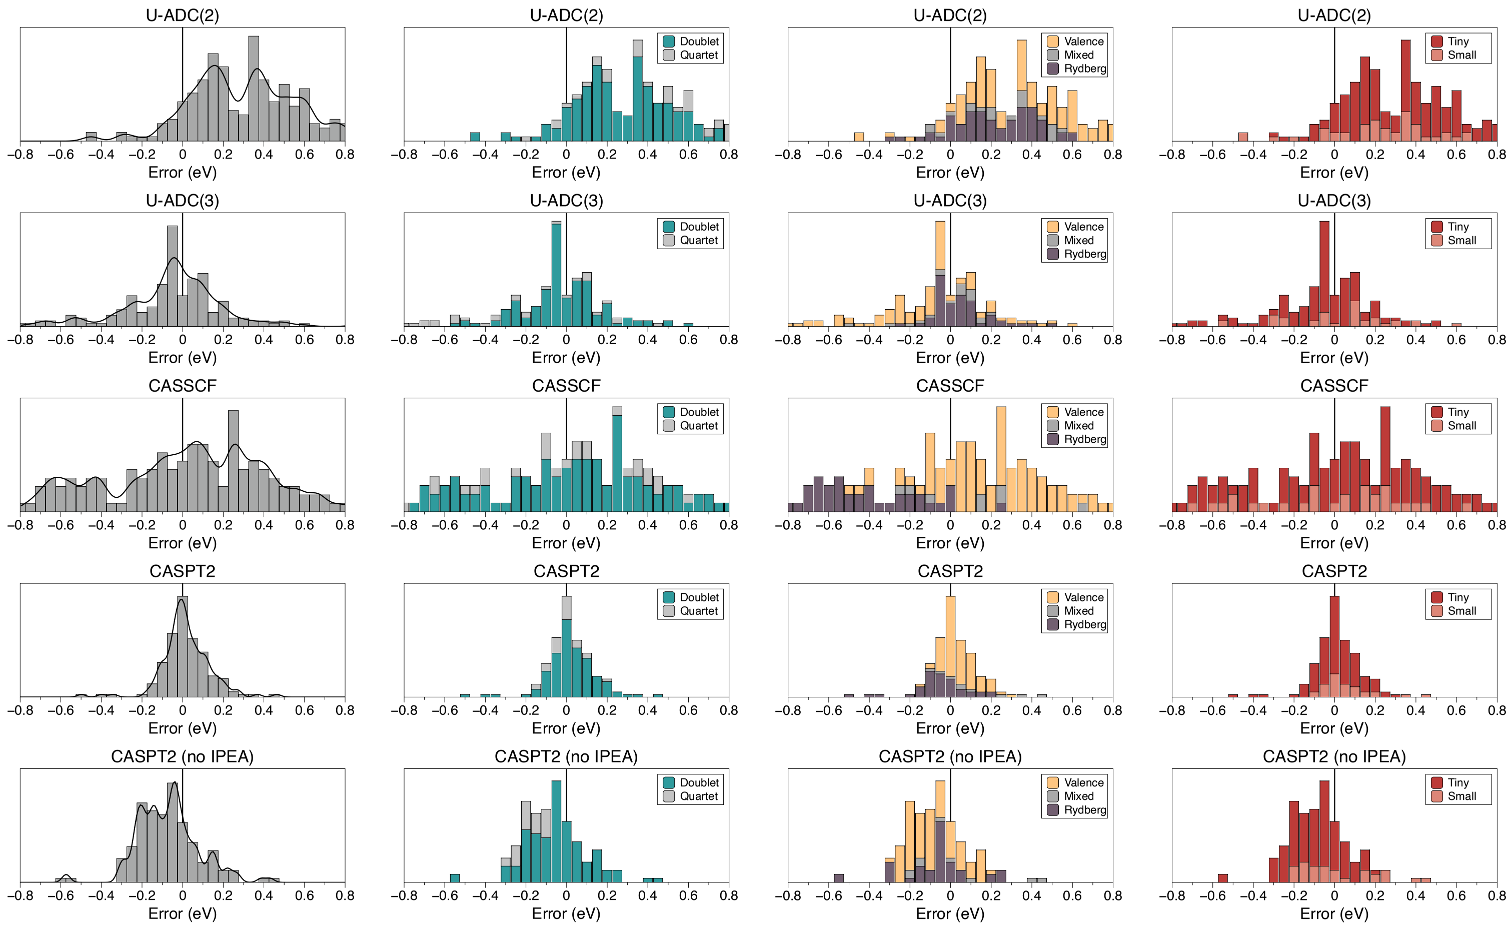


Figure S12: Distribution of the errors on VTEs for selected methods considering all safe and non-GD data in the of RAD subset. From left to right: all transitions, impact of the spin symmetry, influence of molecular size, and effect of ES nature.

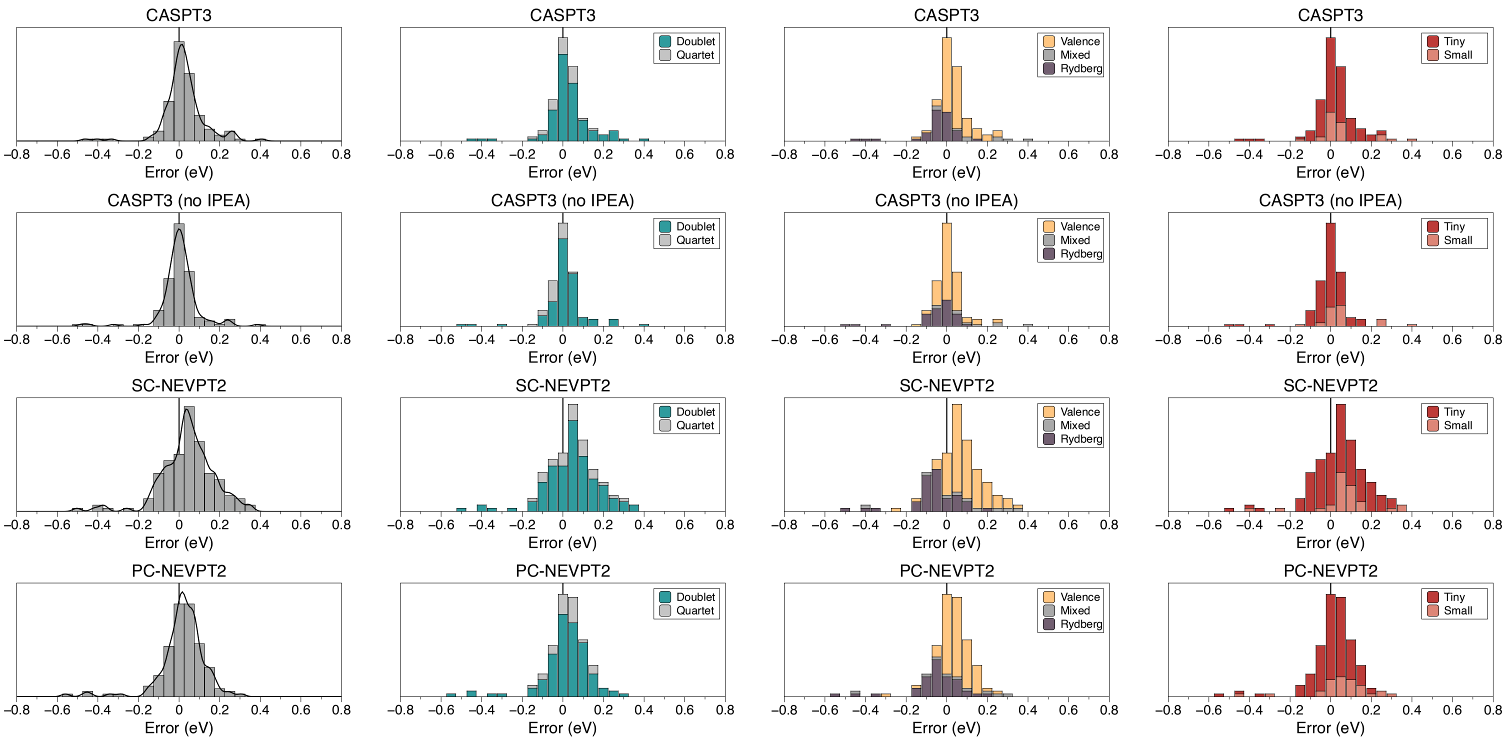


Figure S13: Distribution of the errors on VTEs for selected methods considering all safe and non-GD data in the of RAD subset. From left to right: all transitions, impact of the spin symmetry, influence of molecular size, and effect of ES nature.

# S4 Example of diet set

We provide below an example of a DIET set with 50 excitations across 20 molecules. This set is derived from the MAIN dataset, excluding both unsafe and genuine double excitations (resulting in 824 transitions across 119 molecules).

Table S9: Composition of the sample DIET set.

| Molecule | State | Spin | V/R | Type | TBE/AVTZ |
|---|---|---|---|---|---|
| Aminobenzonitrile | $^1B_2$ | 1 | V | $\pi\pi^\star$ | 4.448 |
| | $^1B_1$ | 1 | R | n.d. | 5.032 |
| | $^1A_1$ | 1 | V | $\pi\pi^\star$ | 5.092 |
| | $^1B_1$ | 1 | R | n.d. | 5.827 |
| Aniline | $^3A_1$ | 3 | V | $\pi\pi^\star$ | 3.951 |
| | $^3B_1$ | 3 | R | n.d. | 5.387 |
| | $^1B_1$ | 1 | R | n.d. | 5.412 |
| | $^1A_1$ | 1 | M | n.d. | 5.494 |
| CCl2 | $^1A_2$ | 1 | V | $n\pi^\star$ | 4.353 |
| Carbon trimer | $^3\Pi_u$ | 3 | V | $n\pi^\star$ | 2.112 |
| | $^1\Delta_u$ | 1 | V | $n\pi^\star$ | 3.962 |
| | $^1\Pi_g$ | 1 | V | $n\pi^\star$ | 4.008 |
| Carbonic acid | $^1A_2$ | 1 | V | $n\pi^\star$ | 7.200 |
| | $^3B_2$ | 3 | R | $n3s$ | 7.481 |
| | $^3B_1$ | 3 | R | $\pi 3s$ | 8.076 |
| | $^1A_1$ | 1 | R | $n3p$ | 8.559 |
| | $^1A_1$ | 1 | V | $\pi\pi^\star$ | 9.251 |
| Chlorobenzene | $^3B_2$ | 3 | V | $\pi\pi^\star$ | 4.723 |
| | $^3B_2$ | 3 | V | $\pi\pi^\star$ | 5.725 |
| | $^1B_1$ | 1 | R | n.d. | 6.307 |
| Cyclopentadienone | $^3A_2$ | 3 | V | $n\pi^\star$ | 2.641 |
| Fluorobenzene | $^1A_1$ | 1 | V | $\pi\pi^\star$ | 6.428 |
| | $^1A_1$ | 1 | V | $\pi\pi^\star$ | 7.202 |
| Furofuran | $^3B_u$ | 3 | V | $\pi\pi^\star$ | 3.565 |
| | $^1A_u$ | 1 | R | n.d. | 5.434 |
| | $^1B_g$ | 1 | R | n.d. | 6.001 |
| | $^1A_g$ | 1 | V | $\pi\pi^\star$ | 6.027 |
| HNC | $^3\Pi$ | 3 | V | $n\pi^\star$ | 6.046 |
| | $^3\Sigma^-$ | 3 | V | $\pi\pi^\star$ | 8.513 |
| | $^1\Delta$ | 1 | V | $\pi\pi^\star$ | 8.795 |
| | $^1\Sigma^+$ | 1 | R | n.d. | 9.658 |
| HSiF | $^1A''$ | 1 | V | $\sigma\pi^\star$ | 3.059 |
| Hexatriene | $^3B_u$ | 3 | V | $\pi\pi^\star$ | 2.734 |
| | $^1A_u$ | 1 | R | $\pi 3s$ | 5.793 |
| Hydrogen peroxide | $^3B$ | 3 | V | $n\sigma$ | 6.035 |
| Imidazole | $^3A'$ | 3 | V | $\pi\pi^\star$ | 4.736 |
| | $^3A''$ | 3 | V | $n\pi^\star$ | 6.309 |
| | $^1A'$ | 1 | R | $\pi 3p$ | 6.391 |
| | $^1A'$ | 1 | R | $n3s$ | 7.039 |
| Nitropyridine N-oxide | $^1A_2$ | 1 | V | $n\pi^\star$ | 3.978 |
| Nitrous acid | $^3A''$ | 3 | V | $n\pi^\star$ | 2.697 |
| | $^1A'$ | 1 | V | $\pi\pi^\star$ | 6.241 |
| | $^3A''$ | 3 | V | $n\pi^\star$ | 6.845 |
| | $^1A'$ | 1 | R | $n3s$ | 7.465 |
| Oxalyl fluoride | $^3B_u$ | 3 | V | $\pi\pi^\star$ | 5.925 |
| | $^1A_g$ | 1 | R | $n3s$ | 8.941 |
| Pentalene ($D_{2h}$) | $^3B_{3g}$ | 3 | V | $\pi\pi^\star$ | 0.384 |
| Triazapentalene | $^1A'$ | 1 | V | $\pi\pi^\star$ | 4.700 |
| | $^1A''$ | 1 | R | n.d. | 4.941 |
| Water | $^1A_2$ | 1 | R | $n3p$ | 9.497 |

Table S10: Statistical results obtained for the sample DIET set as compared to the full training set based on MAIN. All energy values are in eV.

| Method | MAE (sub/full) | MSE (sub/full) | RMSE (sub/full) | # (sub/full) |
|---|---|---|---|---|
| ADC(2) | 0.1804 / 0.1670 | -0.0199 / -0.0274 | 0.2406 / 0.2397 | 50 / 821 |
| ADC(2.5) | 0.0760 / 0.0809 | -0.0465 / -0.0526 | 0.1035 / 0.1116 | 50 / 817 |
| ADC(3) | 0.2230 / 0.2031 | -0.0732 / -0.0790 | 0.2655 / 0.2529 | 50 / 819 |
| CC2 | 0.1739 / 0.1708 | 0.0140 / 0.0072 | 0.2363 / 0.2353 | 50 / 820 |
| CC3 | 0.0229 / 0.0214 | 0.0071 / 0.0059 | 0.0396 / 0.0571 | 50 / 824 |
| CCSD | 0.1336 / 0.1319 | 0.1050 / 0.1139 | 0.1675 / 0.1793 | 50 / 823 |
| CCSD(T)(a)$^{\star}$ | 0.0675 / 0.0621 | 0.0581 / 0.0559 | 0.1008 / 0.0964 | 31 / 521 |
| CCSDR(3) | 0.0624 / 0.0592 | 0.0547 / 0.0536 | 0.0916 / 0.0915 | 31 / 521 |
| CCSDT | 0.0285 / 0.0237 | 0.0031 / 0.0048 | 0.0448 / 0.0710 | 22 / 463 |
| CCSDT-3 | 0.0557 / 0.0557 | 0.0483 / 0.0534 | 0.0732 / 0.0868 | 31 / 522 |
| CIS(D) | 0.2461 / 0.2393 | 0.1329 / 0.1270 | 0.3112 / 0.3157 | 50 / 815 |
| EOM-MP2 | 0.2716 / 0.2727 | 0.2512 / 0.2486 | 0.3120 / 0.3278 | 50 / 823 |
| SCS-CC2 | 0.1697 / 0.1745 | 0.1434 / 0.1417 | 0.2169 / 0.2205 | 50 / 821 |
| SOS-ADC(2) [QC] | 0.1462 / 0.1364 | 0.0137 / 0.0163 | 0.2073 / 0.1942 | 50 / 823 |
| SOS-ADC(2) [TM] | 0.2160 / 0.2133 | 0.1747 / 0.1869 | 0.2681 / 0.2693 | 50 / 823 |
| SOS-CC2 | 0.2230 / 0.2217 | 0.2072 / 0.2090 | 0.2605 / 0.2708 | 50 / 820 |
| STEOM-CCSD | 0.1224 / 0.1152 | -0.0119 / -0.0087 | 0.1382 / 0.1554 | 48 / 723 |
